# Supplementary material for: System size and boundaries determine the patterning dynamics of attracting active particles
Source: arXiv:2509.08533 ancillary file (2025-09-10)
Supplement: Supplementary file 1 [file supplementalmaterials.pdf]

# SUPPLEMENTAL FIGURES

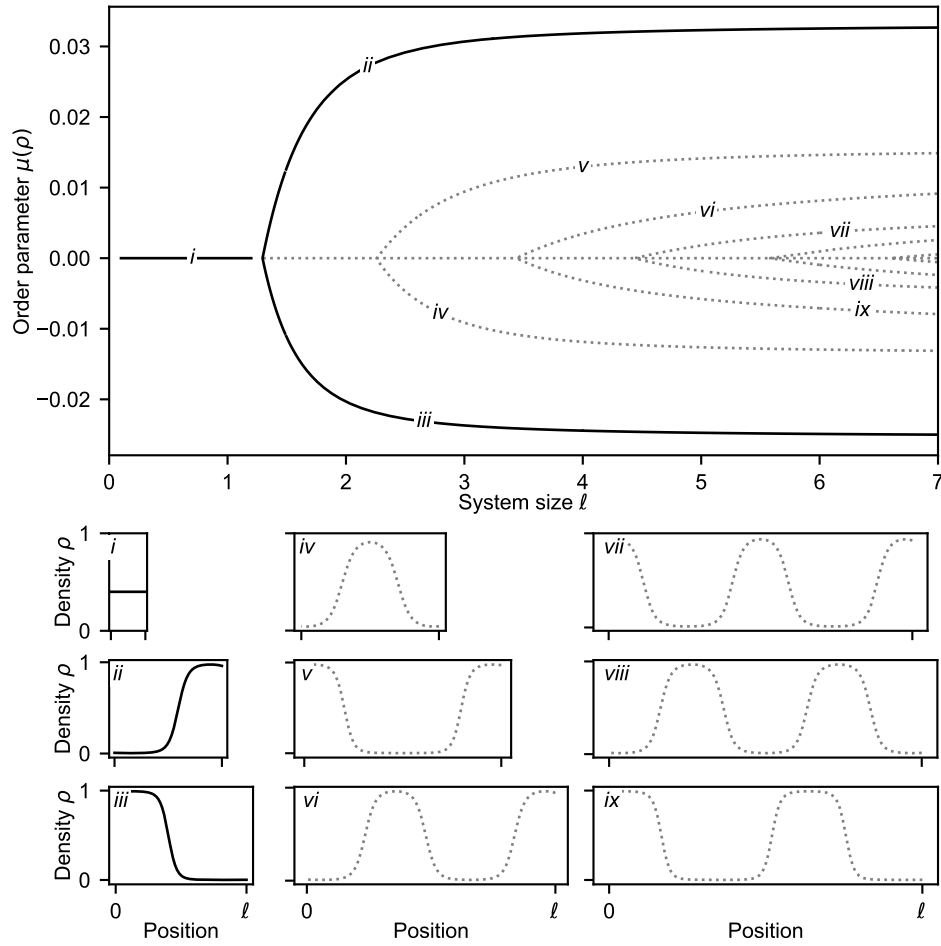

FIG. S1. Bifurcation diagram with steady states as function of cell-cell interaction  $\ell$ . Top top panel is the same as in Fig. 4a in the main text. The density profiles on the bottom correspond to the roman numerals on the branches.

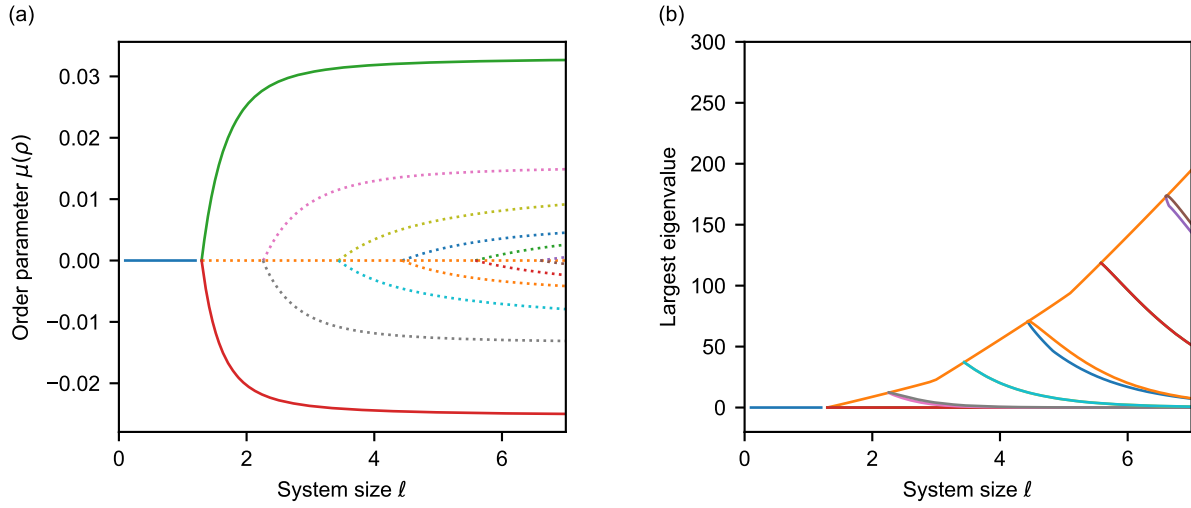

FIG. S2. Bifurcation diagram with steady states as function of system size  $\ell$ . The left panel is the same as Fig. 4a in the main text and Fig. S1. On the right, for each of the branches, the value of the largest eigenvalue of the linearized equation around the steady state is shown. The colors between left and right panels correspond. The largest eigenvalue decreases to zero for each of the branches except the branch with the uniform (flat) density profile.

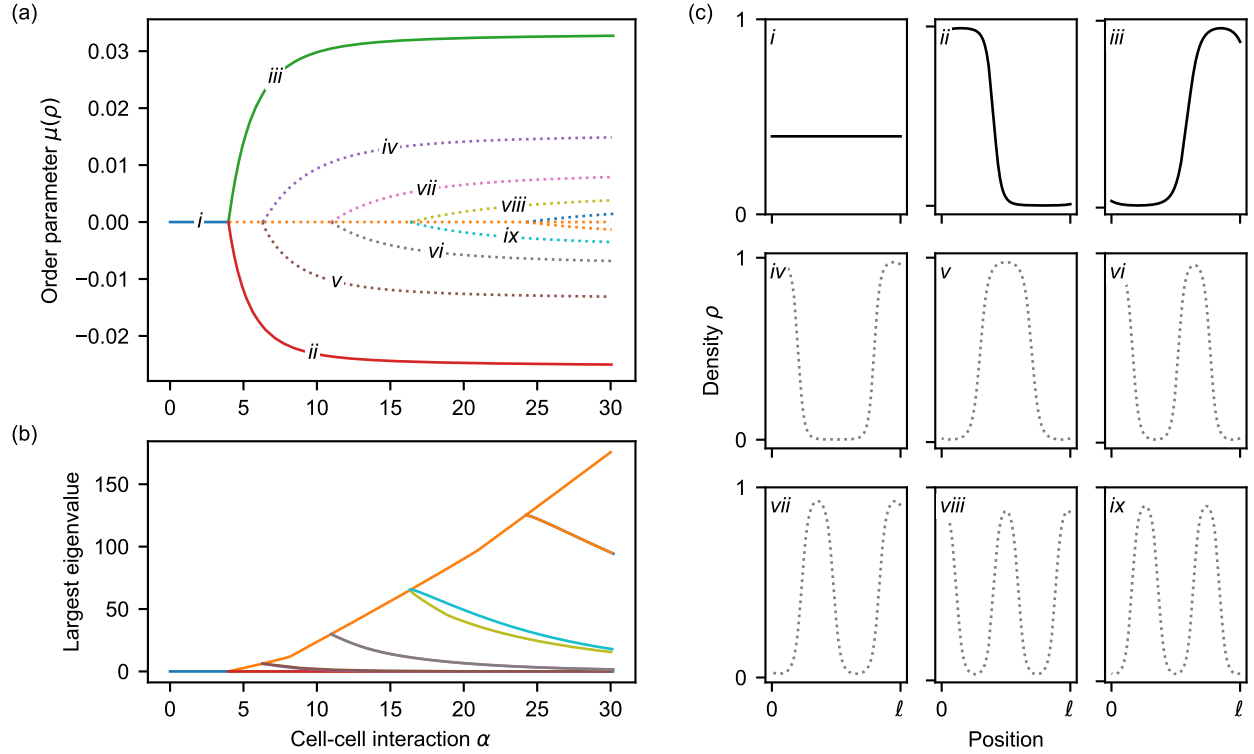

FIG. S3. a) Bifurcation diagram with steady states as function of cell-cell interaction  $\alpha$ . b) The largest eigenvalue of each branch. Colors correspond to the colors in panel a. c) Examples of density profiles. Their location on the branches is indicated by the roman numeral in panel a.

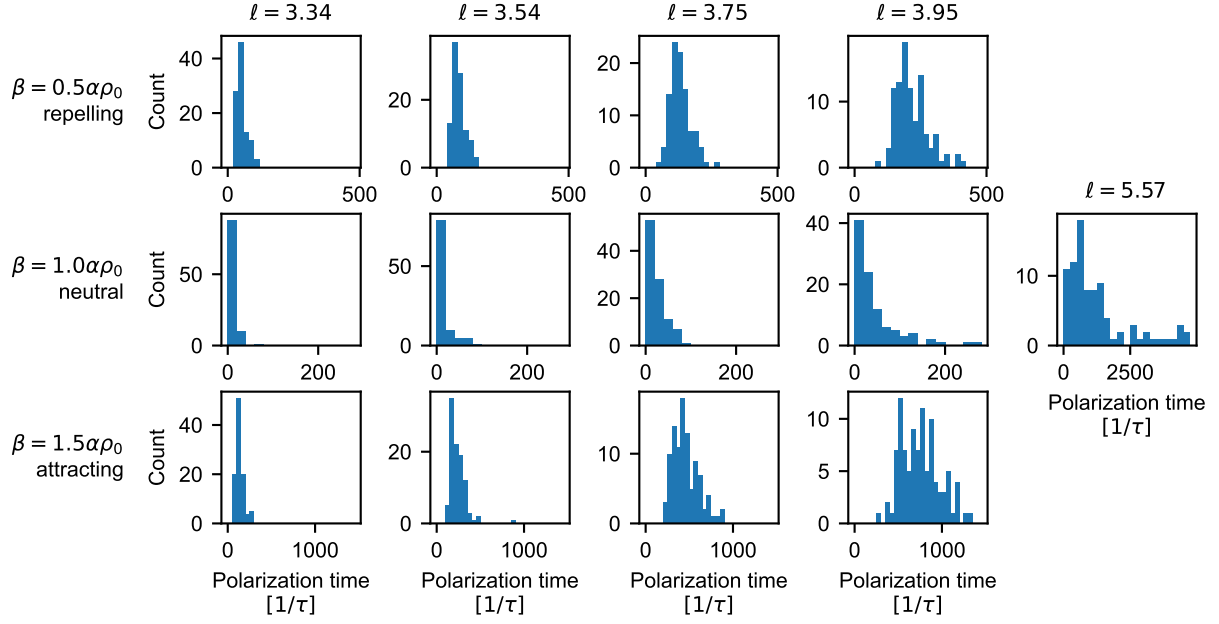

FIG. S4. Distribution of polarization times for selected lengths, and different boundary interactions (repelling, neutral, attracting), corresponding to the summary statistics shown in Fig. 4b in the main text. For the largest length value, the distribution is only shown for neutral boundary effect, since for the others most of the simulations had not polarized by the end of simulation time (5000 time units). Note that for neutral boundary interaction, the distribution looks exponential, which would correspond to the similar scaling for mean and standard deviation observed in Fig. 4b. For larger lengths, the peak of the distribution shifts rightwards also for the neutral boundary interaction.

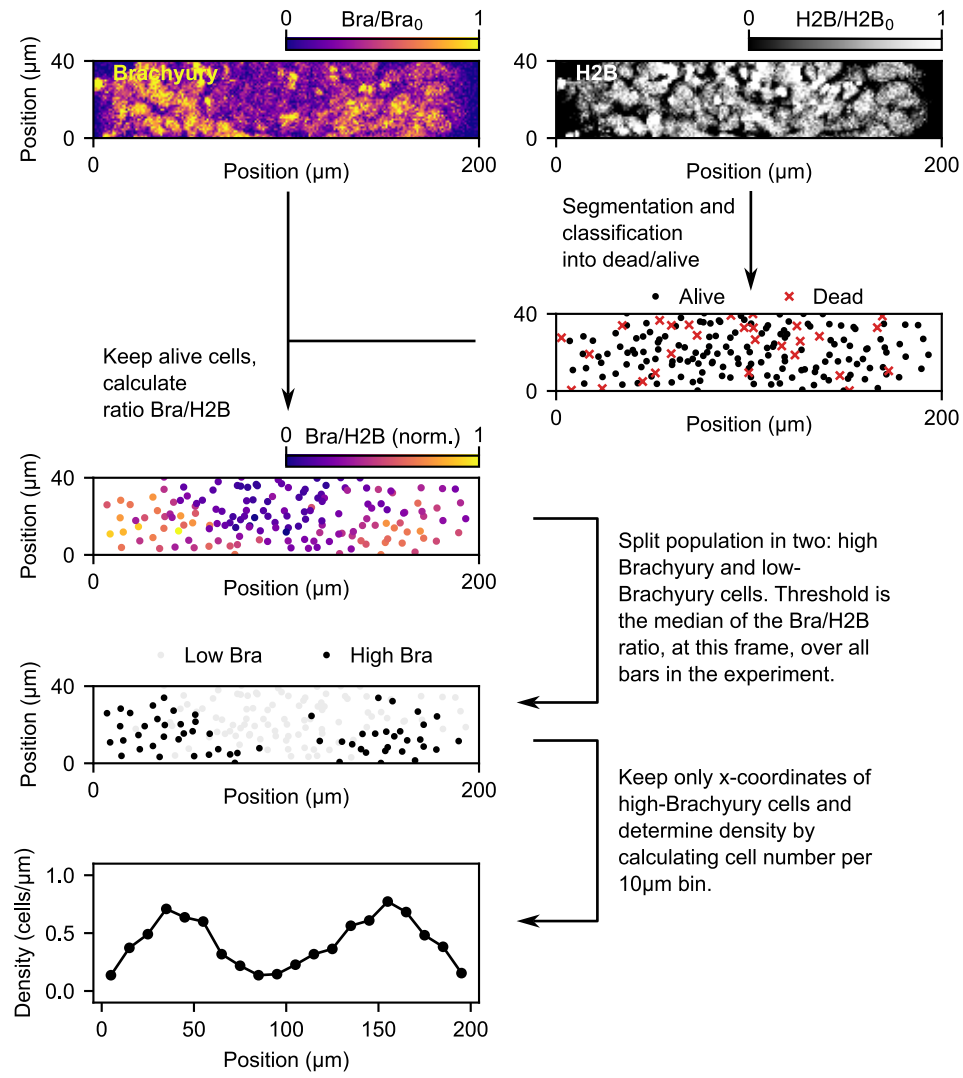

FIG. S5. Workflow for going from image to density profiles.

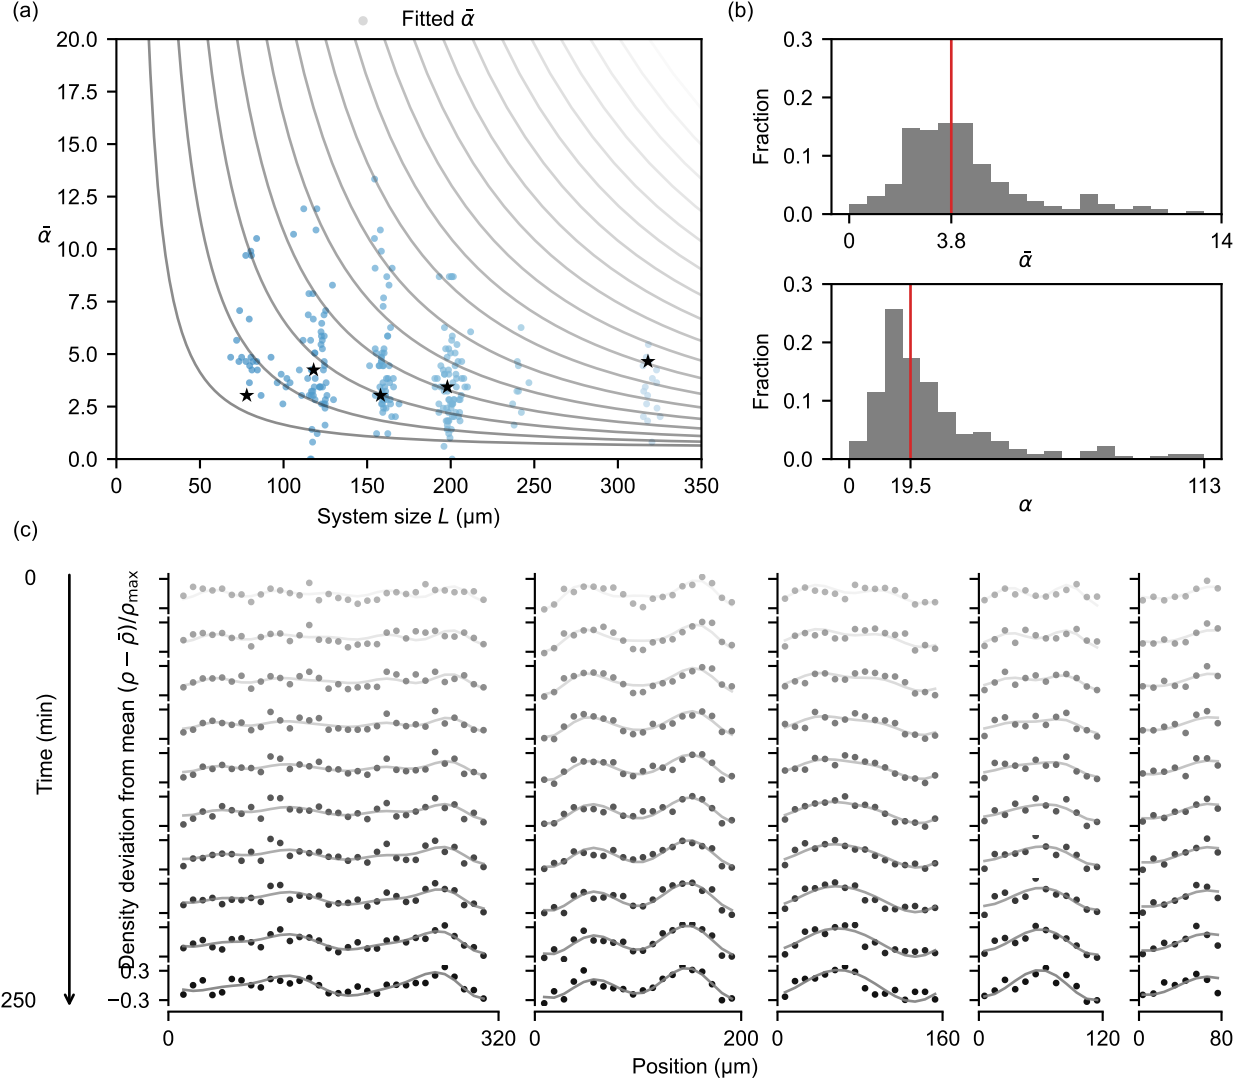

FIG. S6. Details on fitting the model to the data in the initial patterning regime a) All fitted values of  $\bar{\alpha}$ . All bar lengths are values in  $\{80, 100, 120, 160, 200, 320\} \mu\text{m}$ , but we added a jitter to the length to better discriminate the points. Solid lines are the instability curves for the spatial modes. b) Top: histogram of fitted  $\bar{\alpha}$ , bottom: histogram of computed  $\alpha$  by inverting  $\bar{\alpha} = \alpha \rho_0 (1 - \rho_0 / \rho_{\text{max}})$ . We took  $\rho_0$  as the average density of the bar over the time window used for the linear fit, and used a constant value of  $\rho_{\text{max}} = 1.2 \text{ cells}/\mu\text{m}$ , estimated by looking at the maximally obtained densities in all bars. c) Evolution over time in the linear regime of selected examples. The final profiles of  $L = 120, 200, 320 \mu\text{m}$  are shown in the main text. We selected these examples by considering for each lengths bars with fitted  $\bar{\alpha}$  between 3 and 6, initial average densities between 0.3 and 0.6 cells/ $\mu\text{m}$ . In each group, we show the bar with the lowest error from the linear fit.

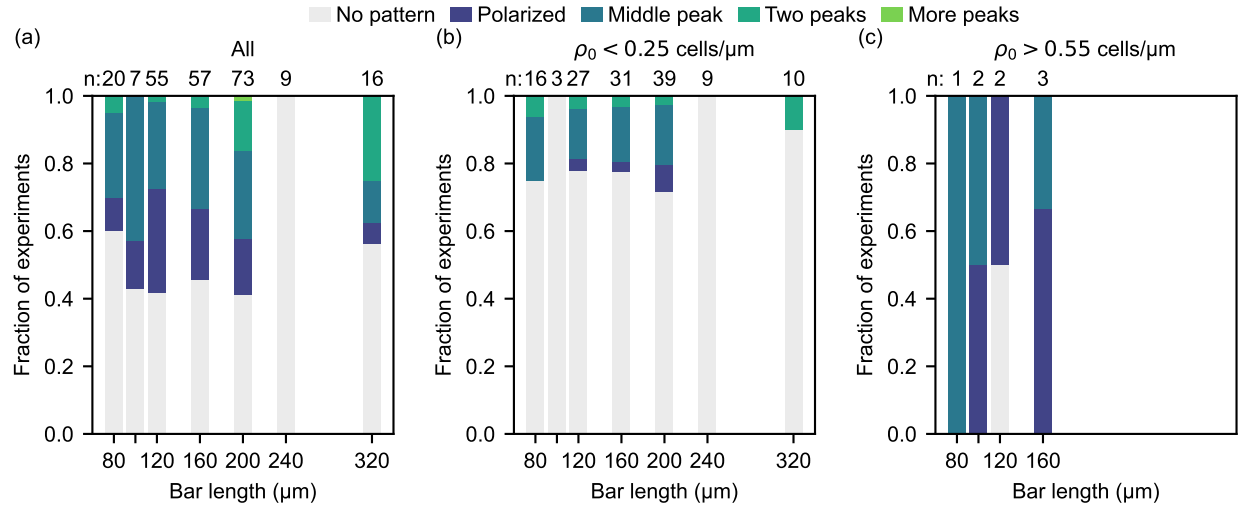

FIG. S7. Classification of the experimentally observed patterns, grouped by the density of the bar. This is the same as Fig. 4e in the main text, which shows the results for  $0.25 < \rho < 0.55$  (cells/ $\mu\text{m}$ ). The left plot shows the results over all experiments, the middle and right for lower and higher densities.

## Experiments

Note: these experiments are part of our companion manuscript [1]. The imaging data will be shared in a repository as part of that paper.

### *Animal Care*

Mice used in all breeding and experiments were housed under veterinarians' supervision in the animal facility at EMBL following the guidelines of the European Commission, revised directive 2010/63/EU and AVMA guidelines 2007. Approval for animal experiments was obtained from the EMBL Institutional Animal Care and Use Committee (project code: 21-001.HD-AA).

### *Mouse Line and Genotyping*

Two mice lines were used in this study: The Brachyury knock-in fluorescent reporter,  $TnEGFP-CreERT2/+$ , was perviously described in [2] and a constitutively expressed fluorescent nuclear marker, R26-H2B-mCherry, was previously generated in [3]. Both fluorescent reporters were maintained together in single mice strain with a primarily CD-1 background and all embryos used were heterozygous for the two transgenic alleles. The detection of a vaginal plug was designated as embryonic day (E) 0.5, and all experiments were conducted with E10.5 embryos. R26-H2B-mCherry was genotyped with primers: (5'-TCCCTCGTGATCTGCAACTCCAGTC-3'), (5'-AACCCAGATGACTACCTATCCTCC-3'), and (5'-GCTGCAGGTCGAGGGACC-3').  $TnEGFP-CreERT2/+$  was genotyped with primers: (5'-GGGCTCTACTTCATCGCATTC -3'), (5'-TATCCCAGTCTCTGGTCTGTGA-3'), and (5'-TAGGACCTACCTAGCAAAGGA-3'). OneTaq 2 X Master Mix with Standard Buffer was used (New England Biolabs) for all polymerase chain reactions.

### *Cell culture and tissue dissociation*

The primary culture media, referred to as "CM", during all imaging experiments consists of DMEM/F12 formulated without glucose, pyruvate, glutamine, and phenol red (Cell Culture Technologies) supplemented with bovine serum albumin (1% w/v, Equitech-Bio), glutamine (2 mM, Sigm-Aldrich), and glucose (2 mM, Sigma-Aldrich) and penicillin/streptomycin (1% v/v, Sigma-Aldrich). A modification is made to the media during embryo dissection and cell dissociation, referred to as "DM", by removing penicillin/streptomycin, reducing the sodium bicarbonate concentration, and adding in 17 mM HEPES (Gibco). Cells used in experiments primarily originate from the tailbud region of E10.5 mouse embryos. To randomize the cells, a piece of a tissue spanning a region between the tip of the tail and the start of the presomitic mesoderm is first cut away from the embryo body with a micro-scalpel. Then the tissue pieces are pooled from 4-10 embryos in 4-6  $\mu$ L of dissection media and mechanically dissociated. The dissociation is done within one well of a circular 4-well silicone micro-insert (Ibidi) by holding the 10  $\mu$ L pipette tip (Gilson) against the wall of the well and gently pushing the tissue pieces back and forth through the small opening. Finally the cell mixture is passed through a 40  $\mu$ m cell strainer (Falcon) to remove large tissue clumps. The filtered mixture is deposited on micropatterned surfaces and incubated at 37°C, 5% CO<sub>2</sub> for  $\sim$  2 hours before the start of imaging.

### *Micropatterning*

One-well chambered glass slides (Cellvis) were prepared by first attaching a rectangular 4-well silicone micro-insert (Ibidi) onto the surface. Then the chambered slide is plasma cleaned for 1.5 minutes and followed by surface passivation with 10  $\mu$ L per well of PLL-*g*-PEG (20  $\mu$ g  $\mu$ L<sup>-1</sup>, SuSoS) for 1 hour at room temperature (22-24 °C). Bars of varying lengths are micropatterned by degradation of the passivation layer with UV light (2400 mJ mm<sup>-2</sup> using the PRIMO patterning system (Aveole). All bar micropatterns have a width of 40  $\mu$ m.

### *Microscopy*

Images were acquired on either Zeiss LSM780 or LSM880 laser scanning confocal microscopes. Image size for one acquisition frame was 512x512 pixels with a pixel size of 0.9225  $\mu$ m. To cover more imaging area, we tiled frames in a

3x3 or 2x4 non-overlapping manner. To excite and capture eGFP and mCherry fluorescence in cells, a 488 nm laser at 1% power setting and a 561 laser at 0.5% power setting was sequentially scanned using a 1.58  $\mu$ s pixel dwell time followed by 2 or 4 times line averaging. The PMT detector gain was set at 800 or 850 with no digital gain or offset used. All samples were imaged in a environmental control box heated to 37°C and supplied with 5% CO<sub>2</sub>. For each experiment, 9-13 z-slices with 2  $\mu$ m spacing were captured at a time interval of 5 minutes per frame for around 16 hours of total imaging time.

### Image Processing

To segment nuclei we trained a StarDist 3D [4] model using hand-annotated training data acquired on different microscopes of the same model using similar imaging settings. The StarDist3D model was trained to segment all bright blob-like objects in single-channel H2B-mcherry images. Afterwards, segmented masks were processed further to classify objects as debris or cell nuclei. Debris was largely characterized by small bright objects from dying cells, but due to variations between experiment days and across z-planes, no simple thresholding strategy could be applied. We instead trained a random-forest classifier for each experiment using the 'Object Classification' workflow available in the Ilastik [5] software package to label objects as debris or nuclei. Training objects were annotated in Ilastik until an acceptable accuracy was achieved as assessed by manual inspection.

## DETAILS ON PROCESSING OF EXPERIMENTAL DATA

### Transforming imaging data into density profiles

To go from the microscopy data to one-dimensional density profiles that can be compared to the theory, we do the following (Fig. S5)

1. Starting from the segmented cell positions, we remove dead cells.
2. We classify each cell as 'high Brachyury' or 'low Brachyury'. The decision is made based on the cell's mean Brachyury intensity divided by its mean H2B intensity. The threshold for determining high/low is the median of the level Bra/H2B for all cells that are on bars, in given experiment, per frame. There is thus a different threshold value for each frame of the experiment, but it is the same for all bars in that experiment.
3. To go from the cell positions to a one-dimensional density profile, we keep only the cell coordinates along the long axis of the bar, and bin these using bins of width 10  $\mu$ m. The density at a point  $x$  is thus the number of cells with coordinate in  $[x - 5, x + 5]$  divided by 10  $\mu$ m.
4. For all further analysis, we smooth the density profiles in time using an 11 point moving average filter.

### Classification of patterns

The pattern classification used in Fig. 5 in the main text is done using a semi-manual heuristic approach based on a decomposition of the density profile into cosine modes.

1. We use the frame corresponding to a timepoint  $t_0 + 800$  minutes, where  $t_0$  is a reference timepoint 200 minutes after plating of the cells.
2. If the average density at this timepoint is too low ( $\bar{\rho} < 0.2$ , we classify as 'no pattern'.
3. Else, we expand the density profile  $\rho_i$  at this timepoint as a cosine series (with wavelengths that are integer multiples of *half* the domain size):

$$\rho_i \approx \sum_{k=0}^K a_k \cos\left(\frac{k\pi}{L}x\right). \quad (1)$$

4. Excluding the constant component  $a_0$ , we determine the two dominant wavenumbers  $k_1$  and  $k_2$  such that  $|a_{k_1}| > |a_{k_2}|$ .



5. If there is a clear difference in contributions between the dominant component and the second-largest, i.e.  $|a_{k_1}| > 1.5|a_{k_2}|$ , then we automatically classify the pattern based on  $k_1$  and sign  $a_{k_1}$ :
  - If  $k_1 = 1$ , the pattern is polarized
  - If  $k_1 = 2$  and  $a_{k_1} < 0$ , we classify as ‘middle peak’.
  - If  $k_1 = 2$  and  $a_{k_1} > 0$ , or if  $k_1 = 3$ , or if  $k_1 = 4$  and  $a_{k_1} < 0$ , we classify as two peaks.
  - In other cases, we classify as multiple peaks.
6. If there is not a clear distinction between the two dominant contributions, we manually check the profile to classify the pattern.

For Fig. 5c, we only show the experimental bars that have density between 0.25 and 0.55 cells/micron. This density is the average of the densities of frames  $t_0 + 750$  to  $t_0 + 800$  minutes with  $t_0$  the timepoint corresponding to 200 minutes after seeding the cells. Fig. S7 shows the same plot, but with all bars included, and the other densities.

### Fitting of $\bar{\alpha}$

We fit the linearized equation to the experimentally observed density time series, in a time interval we identify as the ‘initial patterning interval’, where the linearization applies. For most experiments, the initial density profiles are relative flat, justifying this approach. For each bar, we have values  $\rho_{i,j}$ , where  $i$  indexes space, corresponding to the position  $x_i$ , and  $j$  indexes time, corresponding to timepoints  $t_j$ , with  $i = 1, \dots, N$  and  $j = 1, \dots, M$ .

1. We determine the time interval to use for the fit as follows: we take all  $j$  such that  $t_j \in [t_{\text{start}}, t_{\text{start}} + 250]$  min. The value of  $t_{\text{start}}$  is computed as follows: let  $t_0$  be the timepoint corresponding to 200 minutes after plating of the cells,  $t_{\text{end}}$  the endpoint of the experiment, and let  $t_1$  be  $\text{argmin}_{t \in [t_0, t_{\text{end}}/3]} \text{std} \rho(t)$ . We then set  $t_{\text{start}} = t_1$ . In other words: we say that the initial patterning regimes starts at the timepoint where the standard deviation of  $\rho$  is at its lowest, which intuitively corresponds to the ‘flattest’ density profile. However, we don’t start before  $t_0$  and not after  $t_{\text{end}}/3$ .
2. We rescale space and time. We scale space with  $35\mu\text{m}$  and time with  $\sigma^2/D = 35^2/3 \approx 400$  min:  $\hat{x}_i = x_i/\sigma$ ,  $\hat{t}_j = t_j/\tau$
3. We subtract for each timepoint the average density, i.e.

$$\rho_{i,j} \mapsto \rho_{i,j} - \frac{1}{N} \sum_i \rho_{i,j}.$$

4. To find the optimal  $\bar{\alpha}$ , we use a naive parameter scan: for 100 values of  $\bar{\alpha}$  between 0 and 20, we calculate  $K$  eigenmodes and the associated eigenvalues  $u_k(x), \omega_k$ . We adapt  $K$  based on the length of the bar, we use the rule-of-thumb  $K = \lfloor L/30 \rfloor + 1$ , where  $L$  is the bar length in micron. We do this because we have different number of spatial positions  $x_i$  for different bar lengths and using too much/too few eigenmodes compared to the number of spatial samples affects the fitting procedure.

For a given  $\bar{\alpha}$ , using the  $u$  and  $\omega$ , we fit coefficients  $c_k$  (using standard least-squares) such that

$$E(\bar{\alpha}) = \sum_{i,j,k} \left( c_k e^{\omega_k \hat{t}_j} u_k(\hat{x}_i) - \rho_{i,j} \right)^2 \quad (2)$$

is minimal. We thus choose the coefficients for each mode to minimize distance to the density evolution over the whole time interval.

After performing this computation for different  $\bar{\alpha}$ , we retain  $\bar{\alpha}$  that gives the minimum  $E(\bar{\alpha})$ .

## DETAILS ON NUMERICS

All code was written in Python. Demonstration notebooks, as well as the data and scripts required to generate all figures, can be found on <https://github.com/JanRombouts/rombouts-zhao-patterning>.

### Simulations

We use a finite volume method to discretize space. To compute the nonlinear term, we employ a FFT-based method proposed in Ref. [6]. This method assumes a spatially periodic system. To use it on bounded domains, we embed the interval of length  $[0, \ell]$  in a longer one of length  $[-\ell, 2\ell]$ , calculate the nonlocal terms using the FFT, and then truncate again to  $[0, \ell]$ . The timestepping of the resulting discrete system was done using the `solve_ivp` function from `scipy`, using the BDF method. We ran most parameter scans on the EMBL HPC cluster [7]. In all simulations (except those used for Fig. 4c,e), we initialized the system at the homogeneous density  $\rho(x) = \rho_0$  and added Gaussian noise with mean zero and standard deviation 0.1. The spatial discretization we use depends on the length, generally we use  $N = \max(50, \ell/0.02)$  spatial discretization points.

For Fig. 4, panel a (bottom) in the main text, we performed 100 simulations per parameter value. To determine the polarization timing, we expanded the density profile  $\rho(x)$  at each timepoint in cosine modes:

$$\rho(x) \approx \sum_{k=0}^K a_k \cos\left(\frac{k\pi}{L}x\right).$$

The polarization time is defined as the timepoint from which  $a_1$  is larger (in absolute value) than all other coefficients. In other words, the timepoint where the first cosine mode becomes dominant.

To compute panel (b) from Fig. 4, we simulated the system from various initial conditions of the form

$$\rho(x) = \rho_0 (1 + a_1 \cos(\pi/\ell x) + a_2 \cos(2\pi/\ell x))$$

with added Gaussian noise (standard deviation 0.05), and simulated forward in time. For each resulting trajectory we compute the coefficients  $a_1(t)$  and  $a_2(t)$  by projecting  $\rho(x, t)$  onto a cosine basis. We then compute the velocity vectors in  $a_1, a_2$  space, and using the `griddata` function from `scipy.interpolate` we plot the resulting vector field.

For Fig. 5b, we performed 200 simulations for each parameter value and then classified the patterns in the same way as we classified the experimental density profiles (see above). We took the timepoint  $t = 2.42\tau$ , which using our scaling  $\tau = 35^2/3$  corresponds to roughly 1000 minutes.

### Determination of eigenvalues and eigenmodes

To perform the linear stability analysis, we need to solve the integro-differential eigenvalue problem

$$(\partial_{xx} - \bar{\alpha}\partial_x \mathcal{A})u = \omega u, \quad (\partial_x u - \bar{\alpha}\mathcal{A}u)|_{x \in \{0; \ell\}} = 0. \quad (3)$$

There are multiple ways to do this, one purely numerical and one based on the analytical exact solution.

#### *Discretization of the eigenvalue equation*

This method is used to quickly determine eigenvalues and modes, which we use to do the fitting of  $\bar{\alpha}$  (described above). This method works for any kernel  $g$ .

We discretize the function  $u$  on  $N + 1$  Chebyshev interpolation points on the interval  $[0, \ell]$  [8]. Discretizing in this way, we have matrices  $D$  for  $\partial_x$  and  $A$  for  $\mathcal{A}$ . The eigenvalue equation is

$$(D^2 - \bar{\alpha}DA)u = \omega u \quad (4)$$

with the extra conditions, stemming from the no-flux boundary conditions, that

$$[(D - \bar{\alpha}A)u]_{j \in \{0, N\}} = 0.$$

We implement the extra conditions by considering the generalized eigenvalue problem

$$Mu = \omega Bu, \quad (5)$$

where  $M$  is the matrix  $D^2 - \bar{\alpha}DA$ , but with the first and last row replaced by the first and last row of  $D - \bar{\alpha}A$  respectively, and  $B$  is the identity matrix but with zeros on the first and last row.

The direct numerical method was also used, in combination with pseudo-arclength continuation, to verify the eigenvalue curves shown in Fig. 2a in the main text. In short: Eq. (5) is of the form

$$F(X, \bar{\alpha}) = 0,$$

where  $X = (u_0, \dots, u_N, \omega)$ . We know that the solutions of  $\bar{\alpha} = 0$  are given by  $\omega_n = -(n\pi/L)^2$  with  $u_j = \cos(n\pi x_j/L)$ . We can then continue the eigenvalue loci in the parameter  $(\bar{\alpha}, \omega)$ -plane using pseudo-arclength continuation.

#### Based on the analytical exact solution

For the exponential kernel, we show in Sec. V of these supplementary notes that the eigenvalues are solutions of

$$\begin{aligned} w_1^2 + (2\bar{\alpha} - 1 - \omega)w_1 + \omega &= 0 \\ w_2^2 + (2\bar{\alpha} - 1 - \omega)w_2 + \omega &= 0 \\ \zeta(\sqrt{w_1})\gamma(\sqrt{w_2}) - \zeta(\sqrt{w_2})\gamma(\sqrt{w_1}) &= 0. \end{aligned} \quad (6)$$

in which

$$\zeta(z) = \frac{e^{\frac{\ell z}{2}}}{z-1} - (-1)^n \frac{e^{-\frac{\ell z}{2}}}{z+1} \quad (7)$$

$$\gamma(z) = \frac{e^{-\frac{z\ell}{2}} - (-1)^n e^{\frac{z\ell}{2}}}{z}. \quad (8)$$

In particular, given  $\ell$ ,  $\bar{\alpha}$  and  $n$  (which indicates the parity of the eigenfunction), this set of three algebraic equations can be solved for  $w_1, w_2$  and  $\omega$ , yielding the different eigenvalues.

Given  $\omega$ , the corresponding eigenfunction  $u$  can be constructed as

$$u(x) = A \left( e^{z_1(x-\ell/2)} + (-1)^n e^{-z_1(x-\ell/2)} \right) + B \left( e^{z_2(x-\ell/2)} + (-1)^n e^{-z_2(x-\ell/2)} \right), \quad (9)$$

where  $z_i = \sqrt{w_i}$  (can be complex), and the coefficients  $A$  and  $B$  need to satisfy

$$A\zeta(z_1) + B\zeta(z_2) = 0.$$

We typically do not solve these set of equations for a fixed parameter set. Rather, we computed the eigenvalue curves for fixed  $\ell$ , for increasing  $\bar{\alpha}$  (as shown in Fig. 2a in the main text). We do this by using a pseudo-arclength continuation method, starting for each  $n$  from the value at  $\bar{\alpha} = 0$ , where  $\omega = -(n\pi/\ell)^2$  and  $w_1 = 1, w_2 = \omega$ . Starting from these solutions, we can continue the curve in the  $(\bar{\alpha}, \omega)$ -plane.

#### Bifurcation diagrams

For the bifurcation diagram (Fig. 3, Fig. 4a in the main text, Figs. S3, ??), we use custom Python code for branch-following use pseudo-arclength continuation [9].

To study the steady state solutions of (18), we discretize the spatial density  $\rho(x)$  using Chebyshev interpolation points  $x_i$ . Typically we use  $N + 1 = 301$  interpolation points including the boundaries. For the derivatives, we use the Chebyshev differentiation matrix [8]. The matrix  $A$  corresponding to the integral operator  $\mathcal{A}_0$  has entries

$$A_{ij} = w_j \tilde{g}(x_j - x_i), \quad (10)$$

with  $w_j$  Clenshaw-Curtis integration weights. This is an approximation of

$$\int_0^L \tilde{g}(y - x_i) p_j(y) dy. \quad (11)$$

with  $p_j$  the polynomial that is 1 at  $x_j$  and zero at the other points.

The steady states are after discretization determined by a system of  $N+1$  nonlinear algebraic equations. We replace the first and last equation by equations enforcing the zero-flux boundary conditions. We solve the system of equations using `fsolve` from `scipy`. To track the steady states as parameters change, we implemented a basic pseudo-arclength continuation algorithm [9].

For the 2-parameter bifurcation diagram in Fig. 3a in the main text, we start out with a one-parameter bifurcation diagram using  $\beta$  as parameter and detect the pitchfork bifurcation. We then use the method from [10, Sec. 5.9] to track the bifurcation point as the two parameters  $\alpha$  and  $\beta$  change.

In order to show all branches on the one-parameter bifurcation diagram, we compute an order parameter, essentially projecting the infinite-dimensional spatial profile onto a scalar. First we rescale space such that the density profile is given on the interval  $[0, 1]$ . Then we compute the order parameter as

$$\begin{aligned}\mu(\rho) &= A(\rho) \|\rho - \rho_0\|_2 \\ &= \int_0^1 \left( \frac{1}{2}(x - 1/2) + (x - 1/2)^2 \right) (\rho(x) - \rho_0) dx \\ &\quad \times \left( \int_0^1 (\rho(x) - \rho_0)^2 dx \right)^{1/2}\end{aligned}\tag{12}$$

## MATHEMATICAL DERIVATIONS

### I. SCALING OF THE EQUATION

The one-dimensional version of the advection-diffusion equation is given by

$$\partial_t \rho = \partial_x \left( D \partial_x \rho - \rho \gamma_0^{-1} (1 - \rho / \rho_{\max}) \left[ \chi_p \int_0^L \tilde{G}(y-x) \rho(y) dy + \chi_b \int_{\mathbb{R} \setminus [0, L]} \tilde{G}(y-x) dy \right] \right). \quad (13)$$

The interaction kernel  $\tilde{G}$  is given by

$$\tilde{G}(r) = \text{sign}(r) \frac{1}{\sigma} g(|r|/\sigma), \quad (14)$$

where  $g$  is a function only defined on the positive numbers. We assume the normalization

$$\int_0^\infty g(r) r dr = 1. \quad (15)$$

We now scale the equation by defining

$$\hat{x} = x/\sigma, \quad \tau = \frac{\sigma^2}{D}, \quad \hat{t} = t/\tau, \quad \hat{\rho}(\hat{x}, \hat{t}) = \frac{1}{\rho_{\max}} \rho(\sigma \hat{x}, \tau \hat{t}) = \frac{1}{\rho_{\max}} \rho(x, t) \quad (16)$$

The equation in terms of the hatted variables is then

$$\partial_{\hat{t}} \hat{\rho} = \partial_{\hat{x}\hat{x}} \hat{\rho} - \frac{\sigma}{D\gamma_0} \partial_{\hat{x}} \left( \hat{\rho} (1 - \hat{\rho}) \left[ \chi_p \rho_{\max} \int_0^{L/\sigma} \tilde{g}(\hat{y} - \hat{x}) \hat{\rho}(\hat{y}) d\hat{y} + \chi_b \int_{\mathbb{R} \setminus [0, L/\sigma]} \tilde{g}(\hat{y} - \hat{x}) d\hat{y} \right] \right) \quad (17)$$

where for notational convenience we use  $\tilde{g}(x) = \text{sign}(x)g(x)$ . Now we define

$$\alpha = \frac{\sigma \chi_p \rho_{\max}}{\gamma_0 D}, \quad \beta = \frac{\chi_b \sigma}{\gamma_0 D}, \quad \ell = \frac{L}{\sigma}$$

and drop the hats to get the scaled equation

$$\partial_t \rho = \partial_{xx} \rho - \partial_x \left( \rho (1 - \rho) \left[ \alpha \int_0^\ell \tilde{g}(y-x) \rho(y) dy + \beta \int_{\mathbb{R} \setminus [0, \ell]} \tilde{g}(y-x) dy \right] \right). \quad (18)$$

The no-flux boundary conditions read in full

$$\left[ \partial_x \rho - \rho (1 - \rho) \left( \alpha \int_0^\ell \tilde{g}(x' - x) \rho(x') dx' + \beta \int_{\mathbb{R} \setminus [0, \ell]} \tilde{g}(x' - x) dx' \right) \right]_{x \in \{0, \ell\}} = 0. \quad (19)$$

### II. DERIVATION OF THE NONLOCAL MODEL FOR TWO PDE SYSTEMS

In this section we show that two well-known pattern-forming mechanisms that are typically expressed using PDEs, can be cast into the form of a nonlocal advection equation. We perform the calculation assuming an infinite domain.

This analytical conversion works because of linearity, which means we can use Green's functions methods to write one variable as an integral over the other variable.

In both cases, we find an exponential kernel, and the length scale of the interaction kernel is given in terms of the parameters of the original system.

### A. Keller-Segel chemotaxis model

One of the simplest models for chemotaxis that show pattern formation is the one proposed by Keller and Segel [11, 12]. The two equations of this model read, in one dimension,

$$\partial_t \rho = \partial_x (D \partial_x \rho - \chi_0 \rho \partial_x c) \quad (20)$$

$$\partial_t c = a \rho - b c + D_c \partial_{xx} c. \quad (21)$$

The first equation is an advection-diffusion equation for the cell density. The velocity is proportional to the gradient of the chemical concentration  $c$ . The chemical is produced by cells, degrades with rate  $b$  and diffuses with diffusion coefficient  $D_c$ .

First we scale all variables:

$$\hat{t} = bt, \quad \hat{x} = \sqrt{b/D_c} x, \quad \hat{\rho} = \rho/\rho_0, \quad \hat{c} = cb/(\rho_0 a).$$

Here  $\rho_0$  is a chosen reference density. The scaled equations read, dropping the hats,

$$\partial_t \rho = d \partial_{xx} \rho - \alpha \partial_x (\rho \partial_x c) \quad (22)$$

$$\partial_t c = \rho - c + \partial_{xx} c. \quad (23)$$

We are left with two dimensionless parameters

$$d = D/D_c, \quad \alpha = \frac{\chi_0 \rho_0 a}{D_c b}.$$

Our goal is now to reduce this to a single equation for the density that includes a nonlocal term. We will do this by assuming that the timescale of equilibration of the chemical is small and setting  $\partial_t c = 0$ . This means that  $c$  at any time can be obtained as the solution of

$$\partial_{xx} c - c = -\rho. \quad (24)$$

We explicitly solve this equation and write  $c$  as function of  $\rho$  using Green's function methods. On an infinite domain, Eq. (24) has to be complemented by the conditions that  $c \rightarrow 0$  for  $x \rightarrow \pm\infty$ .

We now compute the Green's function  $G(x, y)$ , which satisfies the equation

$$\partial_{xx} G - G = \delta(x - y) \quad (25)$$

as well as boundary conditions  $G(x, y) \rightarrow 0$  as  $x \rightarrow \pm\infty$ . The Green's function has to be continuous at  $x = y$ , symmetric in its arguments, and  $\partial_x G$  has a jump condition at  $x = y$  given by

$$\partial_x G(x = y^+, y) - \partial_x G(x = y^-, y) = 1$$

With the Green's function known, we can explicitly write the solution to Eq. (24) as

$$c(x) = - \int_{-\infty}^{\infty} G(x, y) \rho(y) dy \quad (26)$$

Let us now solve for  $G$ . Everywhere except at  $x = y$ ,  $G$  satisfies

$$\partial_{xx} G - G = 0,$$

with solution

$$G(x, y) = a(y)e^x + b(y)e^{-x}.$$

The boundary conditions impose that  $a$  is zero for  $x > y$  and  $b = 0$  for  $x < y$ . Therefore we have

$$G(x, y) = \begin{cases} a(y)e^x & x < y \\ b(y)e^{-x} & x > y. \end{cases} \quad (27)$$

continuity at  $x = y$  requires that  $a(y)e^y = b(y)e^{-y}$  such that we can write

$$G(x, y) = \begin{cases} a(y)e^x & x < y \\ a(y)e^{2y-x} & x > y. \end{cases} \quad (28)$$

Next, the jump condition requires that

$$\partial_x G(x = y^+, y) - \partial_x G(x = y^-, y) = 1$$

which gives

$$-a(y)e^y - a(y)e^y = 1 \Rightarrow a(y) = -\frac{1}{2}e^{-y}$$

The Green's function is thus

$$G(x, y) = \begin{cases} -\frac{1}{2}e^{x-y} & x < y \\ -\frac{1}{2}e^{y-x} & x > y. \end{cases} = -\frac{1}{2}e^{-|x-y|}. \quad (29)$$

So, we have that

$$c(x) = \int_{-\infty}^{\infty} \frac{1}{2}e^{-|x-y|}\rho(y)dy. \quad (30)$$

Now, the term in the advective part of the equation for  $\rho$  is proportional to  $\partial_x c$ , which is

$$\partial_x \left( \int_{-\infty}^{\infty} \frac{1}{2}e^{-|x-y|}\rho(y)dy \right) = \int_{-\infty}^{\infty} \frac{1}{2} \text{sign}(y-x)e^{-|x-y|}\rho(y)dy. \quad (31)$$

The nonlocal equivalent of the Keller-Segel model is thus

$$\partial_t \rho = d\partial_{xx}\rho - \partial_x \left( \rho \frac{\alpha}{2} \int_{-\infty}^{\infty} \tilde{g}(y-x)\rho(y)dy \right), \quad (32)$$

with

$$\tilde{g}(y) = \text{sign}(y-x)e^{-|y-x|}.$$

This is exactly the nonlocal advection-diffusion model we are using, with an exponential kernel.

Eq. (32) is in scaled units. Transforming back to the original units gives

$$\partial_t \rho = D\partial_{xx}\rho - \partial_x \left( \frac{\chi_0 a \sigma}{2D_c} \int \frac{1}{\sigma} \text{sign}(y-x)e^{-\frac{|y-x|}{\sigma}} \rho(y)dy \right), \quad (33)$$

where

$$\sigma = \sqrt{\frac{D_c}{b}} \quad (34)$$

is the length scale of the interaction kernel, which in this case is determined by the diffusion and degradation rates of the chemical.

## B. Contractile active matter

This section is based on the equations in Bois *et al.* [13] and Palmquist *et al.* [14] who use them to describe a contractile instability in a molecular and multicellular system respectively. We will interpret the equations in the multicellular context, where they describe a collection of cells that can induce active stresses. From mass and momentum conservation in the low Reynolds number limit, the following equations can be derived:

$$\partial_t \rho = \partial_x (D\partial_x \rho - v\rho) \quad (35)$$

$$0 = -\gamma v + \partial_x \sigma. \quad (36)$$

The first equation describes the evolution of cell density  $\rho$ , affected by diffusion and advection in a velocity field  $v$ . The second equation describes the balance of forces in the material. Here  $\sigma(x)$  is the stress and the term  $\gamma v$  corresponds to the friction force with a substrate.

The stress has two components, a viscous stress  $\eta \partial_x v$  and an active force generated by the contractile cells. We assume that this stress is proportional to cell density,  $\sigma_A = b\rho$ . This leads to

$$\partial_t \rho = \partial_x (D \partial_x \rho - v \rho) \quad (37)$$

$$0 = -\gamma v + \partial_x (\eta \partial_x v + b\rho). \quad (38)$$

We scale the equations first. The scaling

$$\hat{x} = \sqrt{\gamma/\eta} x, \quad \hat{\rho} = \rho/\rho_0, \quad \hat{v} = \frac{\sqrt{\gamma\eta}}{b\rho_0} v, \quad \hat{t} = \frac{D\gamma}{\eta} t$$

yields the equations (dropping hats)

$$\partial_t \rho = \partial_{xx} \rho - \alpha \partial_x (\rho v) \quad (39)$$

$$0 = -v + \partial_{xx} v + \partial_x \rho. \quad (40)$$

With a single parameter

$$\alpha = \frac{b\rho_0}{D\gamma}, \quad (41)$$

corresponding to a Péclet number.

The second equation is an ODE for  $v$  in space. There is no time derivative because we neglect inertial forces (low Reynolds number limit). The equation can be written

$$\partial_{xx} v - v = -\partial_x \rho,$$

which is of the same form as Eq. (24) for the chemical concentration in the Keller-Segel example. Using the same Green's function method — with the condition that  $v(\pm\infty) = 0$ , we immediately write down

$$v(x) = \int_{-\infty}^{\infty} \frac{1}{2} e^{-|x-y|} \partial_y \rho(y) dy.$$

Integration by parts yields (the boundary terms drop out)

$$v(x) = \int_{-\infty}^{\infty} \frac{1}{2} \text{sign}(y-x) e^{-|x-y|} \rho(y) dy,$$

which can be directly plugged into the equation for  $\rho$ :

$$\partial_t \rho = \partial_{xx} \rho - \alpha \partial_x \left( \rho \int \frac{1}{2} \text{sign}(y-x) e^{-|x-y|} \rho(y) dy \right). \quad (42)$$

This is the expected nonlocal formulation of this model, with an exponentially decaying interaction kernel.

Rewriting it back with physical units yields

$$\partial_t \rho = D \partial_{xx} \rho - \frac{b}{2\sqrt{\eta\gamma}} \partial_x \left( \rho \int \frac{1}{\sigma} \text{sign}(y-x) e^{-\frac{|y-x|}{\sigma}} \rho(y) dy \right) \quad (43)$$

where the length scale is

$$\sigma = \sqrt{\frac{\eta}{\gamma}}.$$

This quantity is known as the hydrodynamic length scale.



### III. LINEAR STABILITY FOR AN INFINITE DOMAIN

Here, we summarize the linear stability analysis for a one-dimensional infinite domain. See the paper by Jewell *et al.* [15] for a more extensive treatment in  $N$  dimensions.

On an infinite domain, the equation has no boundary interaction term and reads, in scaled units,

$$\partial_t \rho = \partial_{xx} \rho - \alpha \partial_x \left( \rho(1 - \rho) \int_{-\infty}^{\infty} \tilde{g}(y - x) \rho(y) dy \right). \quad (44)$$

Any constant solution  $\rho(x) = \rho_0$  is a steady state. We linearize around  $\rho_0$  by setting  $\rho(x, t) = \rho_0 + \tilde{\rho}(x, t)$  with  $\tilde{\rho}$  a small perturbation. Keeping only terms linear in  $\tilde{\rho}$  gives

$$\partial_t \tilde{\rho} = \partial_{xx} \tilde{\rho} - \bar{\alpha} \partial_x \left( \int_{-\infty}^{\infty} \tilde{g}(y - x) \tilde{\rho}(y) dy \right), \quad (45)$$

where we have set  $\bar{\alpha} = \alpha \rho_0 (1 - \rho_0)$ . Here, we have used that

$$\int_{-\infty}^{\infty} \tilde{g}(y - x) dy = 0.$$

In order to continue, we assume that  $\tilde{\rho}(x, t) = e^{\omega t + i k x}$  to derive the dispersion relation. First, we have

$$\partial_x \left( \int_{-\infty}^{\infty} \tilde{g}(y - x) e^{i k y} dy \right) = \partial_x \left( \int_{-\infty}^{\infty} \tilde{g}(s) e^{i k (x+s)} ds \right) \quad (46)$$

where we have used the translation invariance on an infinite domain in the first equation (this does not work on finite domains). Next, we compute, using  $\tilde{g}(s) = \text{sign}(s)g(|s|)$ :

$$\partial_x \left( \int_{-\infty}^{\infty} \tilde{g}(s) e^{i k (x+s)} ds \right) = i k e^{i k x} \int_{-\infty}^{\infty} \tilde{g}(s) e^{i k s} ds \quad (47)$$

$$= i k e^{i k x} \left( \int_{-\infty}^0 -g(-s) e^{i k s} ds + \int_0^{\infty} g(s) e^{i k s} ds \right) \quad (48)$$

Changing the integration variable in the first integral from  $s$  to  $-s$ , and switching the integration limits, gives

$$i k e^{i k x} \left( \int_{-\infty}^0 -g(-s) e^{i k s} ds + \int_0^{\infty} g(s) e^{i k s} ds \right) = i k e^{i k x} \left( - \int_0^{\infty} g(s) e^{-i k s} ds + \int_0^{\infty} g(s) e^{i k s} ds \right) \quad (49)$$

$$= i k e^{i k x} \int_0^{\infty} g(s) 2i \sin(k s) ds \quad (50)$$

$$= -2k e^{i k x} \hat{g}^s(k) \quad (51)$$

where  $\hat{g}^s$  is the Fourier sine transform of  $g$ . So, plugging in  $\tilde{\rho} = e^{\omega t + i k x}$  and cancelling the exponentials in Eq. (45) yields

$$\omega = -k^2 + 2\bar{\alpha} k \hat{g}^s(k). \quad (52)$$

This is the dispersion relation, linking the growth rate  $\omega$  of a spatial mode to its wavenumber  $k$ . An instability leading to patterns exists if there are  $k$  such that  $\omega(k) > 0$ .

In the particular case of  $g(x) = e^{-x}$ , we can compute  $\hat{g}^s(k)$  explicitly:

$$\int_0^{\infty} e^{-x} \sin(k x) dx = \frac{k}{k^2 + 1}. \quad (53)$$

The dispersion relation is thus

$$\omega = -k^2 + 2\bar{\alpha} \frac{k^2}{k^2 + 1}. \quad (54)$$

By computing the maximum of this function, we find that there is only a positive  $\omega$  if  $\bar{\alpha} > 1/2$ .

#### IV. ANALYSIS OF THE EIGENVALUE EQUATION ON BOUNDED DOMAINS

The eigenvalue problem that arises from the linear stability analysis on bounded domains is given by

$$(\partial_{xx} - \bar{\alpha}\partial_x\mathcal{A})u = \omega u, \quad \partial_x u - \bar{\alpha}\mathcal{A}u = 0 \text{ at } x = 0, \ell., \quad (55)$$

where

$$(\mathcal{A}u)(x) = \int_0^\ell \tilde{g}(y-x)u(y)dy. \quad (56)$$

##### A. Parity of the eigenfunctions

First we show that the solutions of Eq. (55) are odd or even around  $x = \ell/2$ .

We show that if  $u(x)$  is a solution of Eq. (55), then  $u(L-x)$  too. Define  $v(x) = u(\ell-x)$ . We have that  $\partial_x v(x) = -(\partial_x u)(\ell-x)$ . For the operator  $\mathcal{A}$ :

$$\begin{aligned} \mathcal{A}(v)(x) &= \int_0^\ell \tilde{g}(y-x)v(y)dy \\ &= \int_0^\ell \tilde{g}(y-x)u(\ell-y)dy \\ &= -\int_\ell^0 \tilde{g}(\ell-z-x)u(z)dz \\ &= \int_0^L \tilde{g}(\ell-x-z)u(z)dz \\ &= \int_0^L \tilde{g}(-(z-(\ell-x)))u(z)dz \\ &= -\int_0^L \tilde{g}(z-(\ell-x))u(z)dz \\ &= -\mathcal{A}(u)(L-x) \end{aligned}$$

We have used here that  $\tilde{g}(-r) = -\tilde{g}(r)$ . This means that

$$(\partial_x - \bar{\alpha}\mathcal{A})(v)(x) = -(\partial_x - \bar{\alpha}\mathcal{A})(u)(L-x).$$

An extra  $x$  derivative switches the sign such that

$$(\partial_{xx} - \bar{\alpha}\partial_x\mathcal{A})(v)(x) = (\partial_{xx} - \bar{\alpha}\partial_x\mathcal{A})(u)(L-x).$$

This means that if  $u(x)$  is an eigenfunction with eigenvalue  $\omega$ , then  $v$  is also one with the same eigenvalue. Assuming the eigenvalues are non-degenerate, this means that  $v(x) = cu(x)$ . Therefore,

$$u(\ell-x) = cu(x) = c^2u(\ell-x),$$

such that  $c = \pm 1$ . This means the eigenfunctions have definite parity, and either even or odd around  $x = \ell/2$ .

**Remark 1** *The fact that the eigenfunctions are odd/even implies that only the boundary condition at one side is sufficient, which will then imply the other. If  $u$  is even, with  $v(x) = u(L-x) = u(x)$ ,*

$$(\partial_x - \bar{\alpha}\mathcal{A})(u)(x=0) = -(\partial_x - \bar{\alpha}\mathcal{A})(v)(x=L) = -(\partial_x - \bar{\alpha}\mathcal{A})(u)(x=L) = 0$$

*and analogously for  $u$  odd.*

### B. For a range of interaction kernels, the eigenfunctions satisfy an ODE

We introduce the following notation for functions and operators:

$$g_m^a = ag_m(ax) = a^{m+1}x^m e^{-ax}, \quad (57)$$

and

$$\mathcal{A}_m^a : u \mapsto \int_0^\ell \text{sign}(y-x) g_m^a(|y-x|) dy \quad (58)$$

In the rest of the section, we will show that for operators that are linear combinations of the ones above, the integro-differential eigenvalue equation can be turned into an ordinary differential equation (Eq. (92)).

#### 1. Properties of the functions $g_m^a$

We set  $g_m(x) = g_m^1(x) = x^m e^{-x}$ . These functions satisfy the following identities for  $m \geq 2$ :

$$g'_m(x) = mx^{m-1}e^{-x} - x^m e^{-x} = mg_{m-1}(x) - g_m(x)$$

and therefore

$$g''_m = (mg_{m-1} - g_m)' \quad (59)$$

$$= mg'_{m-1} - g'_m \quad (60)$$

$$= m(m-1)g_{m-2} - mg_{m-1} - mg_{m-1} + g_m \quad (61)$$

$$= m(m-1)g_{m-2} - 2mg_{m-1} + g_m \quad (62)$$

For  $m = 0$ , the exponential case, we have

$$g'_0 = -g_0, \quad g''_0 = g_0$$

For  $m = 1$ , we have

$$g'_1 = e^{-x} - xe^{-x}, \quad g''_1 = -e^{-x} - e^{-x} + xe^{-x}$$

This means that Eq. (62) also holds for  $m = 0$  and  $m = 1$ , because of the multiplications with  $m$  and  $m - 1$  terms like  $g_{-1}$  drop out.

Finally we note that when evaluating at  $x = 0$ , only the  $m = 0$  function is non zero:

$$g_m(0) = \delta_m.$$

From this calculation for  $a = 1$ , we derive immediately for general  $a$ , since  $g_m^a(x) = ag_m^1(ax)$ :

$$(g_m^a)'' = a^2 [m(m-1)g_{m-2}^a - 2mg_{m-1}^a + g_m^a]. \quad (63)$$

#### 2. A recursion relation for the operator $\mathcal{A}_m^a$

We now show that the properties of the functions  $g_m^a$  translate into the following relation for the integral operators using  $g_m^a$  as kernel:

$$(a^{-2}\partial_{xx} - 1)\mathcal{A}_m^a u = m(m-1)\mathcal{A}_{m-2}^a u - 2m\mathcal{A}_{m-1}^a u - 2a^{-1}\delta_m\partial_x u \quad (64)$$

We calculate  $\partial_{xx}\mathcal{A}_m^a u$ . We first split the integral to get rid of the absolute values:

$$\mathcal{A}_m^a u = -\int_0^x g_m^a(x-y)u(y)dy + \int_x^\ell g_m^a(y-x)u(y)dy. \quad (65)$$

Now, we take the  $x$ -derivative of this, using Leibniz' chain rule for integrals. This gives

$$\partial_x \mathcal{A}_m^a u = -g_m^a(0)u(x) - \int_0^x (g_m^a)'(x-y)u(y)dy - g_m^a(0)u(x) - \int_x^\ell (g_m^a)'(y-x)u(y)dy \quad (66)$$

$$= - \int_0^x (g_m^a)'(x-y)u(y)dy - \int_x^\ell (g_m^a)'(y-x)u(y)dy - 2g_m^a(0)u(x). \quad (67)$$

Deriving with respect to  $x$  once more then gives

$$\partial_{xx} \mathcal{A}_m^a u = -(g_m^a)'(0)u(0) - \int_0^x (g_m^a)''(x-y)u(y)dy + (g_m^a)'(0)u(x) + \int_x^\ell (g_m^a)''(y-x)u(y)dy - 2g_m(0)u'(x) \quad (68)$$

$$= - \int_0^x (g_m^a)''(x-y)u(y)dy + \int_x^\ell (g_m^a)''(y-x)u(y)dy - 2g_m^a(0)u'(x) \quad (\star)$$

Now we use the identities for the derivatives of the function  $g_m^a$  and recombine the integrals:  $(\star)$  is equal to

$$-a^2 \int_0^x (m(m-1)g_{m-2}^a - 2mg_{m-1}^a + g_m^a)(x-y)u(y)dy \quad (69)$$

$$+ a^2 \int_x^\ell (m(m-1)g_{m-2}^a - 2mg_{m-1}^a + g_m^a)(y-x)u(y)dy - 2g_m^a(0)u'(x). \quad (70)$$

Combining for each  $g_m$  the two integrals, we find

$$\partial_{xx} \mathcal{A}_m^a u = a^2 [m(m-1)\mathcal{A}_{m-2}^a u - 2m\mathcal{A}_{m-1}^a u + \mathcal{A}_m^a u] - 2\delta_m a \partial_x u, \quad (71)$$

which is equivalent to Eq. (64). We also used that  $g_m^a(0) = \delta_m a$ .

### 3. Repeatedly applying $a^{-2}\partial_{xx} - 1$ to $\mathcal{A}_m^a$ gives a differential operator

From Eq. (64), we see that applying the operator  $a^{-2}\partial_{xx} - 1$  after the integral operator  $\mathcal{A}_m^a$  leads to an expression with only integral operators with lower  $m$ , as well as a differential operator. Moreover, applying  $a^{-2}\partial_{xx} - 1$  to  $\mathcal{A}_0^a$  gives  $-2a^{-1}\partial_x$ . Thus, applying  $a^{-2}\partial_{xx} - 1$  a total of  $m+1$  times after  $\mathcal{A}_m^a$  should only leave an operator involving derivatives:

$$(a^{-2}\partial_{xx} - 1)^{m+1} \mathcal{A}_m^a u = \mathcal{L}_m^a u \quad (72)$$

with  $\mathcal{L}_m^a$  an as-of-yet unspecified differential operator. We will now derive a recursion for this operator and then solve it. For notational convenience, we define the rescaled derivative operator

$$\mathcal{D}_a = a^{-1}\partial_x. \quad (73)$$

With this notation, Eq. (64) is written as

$$(\mathcal{D}_a^2 - 1)\mathcal{A}_m u = m(m-1)\mathcal{A}_{m-2}^a u - 2m\mathcal{A}_{m-1}^a u - 2\delta_m \mathcal{D}_a u \quad (74)$$

We have:

$$\mathcal{L}_m^a u = (\mathcal{D}_a^2 - 1)^{m+1} \mathcal{A}_m^a u \quad (75)$$

$$= (\mathcal{D}_a^2 - 1)^m (\mathcal{D}_a^2 - 1) \mathcal{A}_m^a u \quad (76)$$

$$= (\mathcal{D}_a^2 - 1)^m (m(m-1)\mathcal{A}_{m-2}^a u - 2m\mathcal{A}_{m-1}^a u - 2\delta_m \mathcal{D}_a u) \quad (77)$$

$$= m(m-1)(\mathcal{D}_a^2 - 1)(\mathcal{D}_a^2 - 1)^{m-1} \mathcal{A}_{m-2}^a u - 2m\mathcal{L}_{m-1}^a u - 2\delta_m (\mathcal{D}_a^2 - 1)^m \mathcal{D}_a u \quad (78)$$

$$= m(m-1)(\mathcal{D}_a^2 - 1)\mathcal{L}_{m-2}^a u - 2m\mathcal{L}_{m-1}^a u - 2\delta_m \mathcal{D}_a u \quad (79)$$

The operators for the first few values of  $m$  are

$$\mathcal{L}_0^a = (\mathcal{D}_a^2 - 1)\mathcal{A}_0^a = -2\mathcal{D}_a \quad (= -2a^{-1}\partial_x) \quad (80)$$

$$\mathcal{L}_1^a = (\mathcal{D}_a^2 - 1)^2 \mathcal{A}_1^a = 4\mathcal{D}_a \quad (= 4a^{-1}\partial_x) \quad (81)$$

$$\mathcal{L}_2^a = (\mathcal{D}_a^2 - 1)^3 \mathcal{A}_2^a = -4\mathcal{D}_a^3 - 12\mathcal{D}_a \quad (82)$$

$$\mathcal{L}_3^a = (\mathcal{D}_a^2 - 1)^4 \mathcal{A}_3^a = 48\mathcal{D}_a^3 + 48\mathcal{D}_a \quad (83)$$

$$\mathcal{L}_4^a = (\mathcal{D}_a^2 - 1)^5 \mathcal{A}_4^a = -48\mathcal{D}_a^5 - 480\mathcal{D}_a^3 - 240\mathcal{D}_a \quad (84)$$

$$\mathcal{L}_5^a = (\mathcal{D}_a^2 - 1)^6 \mathcal{A}_5^a = 1440\mathcal{D}_a^5 + 4800\mathcal{D}_a^3 + 1440\mathcal{D}_a. \quad (85)$$

The explicit solution for  $\mathcal{L}_m^a$  is

$$\mathcal{L}_m^a(u) = m!(-1)^{m+1}2 \sum_{k=0}^{\lfloor m/2 \rfloor} \binom{m+1}{2k+1} \mathcal{D}_a^{2k+1} u. \quad (86)$$

A slightly simpler expression is

$$\mathcal{L}_m^a = m!(-1)^{m+1} \left( (1 + \mathcal{D}_a)^{m+1} - (1 - \mathcal{D}_a)^{m+1} \right). \quad (87)$$

This can be checked by substituting these formulas into the recursion equation.

The degree of  $\mathcal{L}_m^a$  is  $m$  if  $m$  is odd and  $m+1$  if  $m$  is even.

#### 4. Reduction for combinations of integral operators

The property in Eq. (72) can be generalized to linear combinations of operators  $\mathcal{A}_m^a$ . Let us define

$$\mathcal{A} = \sum_{i=1}^n c_i \mathcal{A}_{m_i}^{a_i}.$$

Then

$$\prod_{j=1}^n (\mathcal{D}_{a_j}^2 - 1)^{m_j+1} \mathcal{A} = \prod_{j=1}^n (\mathcal{D}_{a_j}^2 - 1)^{m_j+1} \left[ \sum_{i=1}^n c_i \mathcal{A}_{m_i}^{a_i} \right] \quad (88)$$

$$= \sum_{i=1}^n c_i \left[ \prod_{j=1}^n (\mathcal{D}_{a_j}^2 - 1)^{m_j+1} \mathcal{A}_{m_i}^{a_i} \right] \quad (89)$$

$$= \sum_{i=1}^n c_i \left[ \prod_{j=1, j \neq i}^n (\mathcal{D}_{a_j}^2 - 1)^{m_j+1} \mathcal{L}_{m_i}^{a_i} \right]. \quad (90)$$

We have used that operators of the form  $\mathcal{D}^2 - 1$  commute with each other. The last expression is a (admittely complicated) differential operator of degree

$$\sum_{i=1}^n 2m_i + 2 + \deg \mathcal{L}_{m_i}^{a_i},$$

so maximally (if all the  $m_i$  are even) this is

$$\sum_{i=1}^n 2m_i + 2 + m_i + 1 = 3 \sum_{i=1}^n (m_i + 1).$$

In particular, if all the operators are defined by exponentials ( $m = 0$ ), the total degree of the operator is  $3n$ .

#### 5. Reducing the integrodifferential eigenvalue equation to an ODE

After all this algebra, we are ready to transform the eigenvalue equation

$$(\partial_{xx} - \bar{\alpha} \partial_x \mathcal{A})u = \omega u$$

into an ODE. We assume that

$$\mathcal{A} = \sum_{i=1}^n c_i \mathcal{A}_{m_i}^{a_i}.$$

We rewrite the eigenvalue equation as

$$(\partial_{xx} - \omega)u = \bar{\alpha}\partial_x \mathcal{A}u.$$

Now, we apply the operator

$$\prod_{j=1}^n (\mathcal{D}_{a_j}^2 - 1)^{m_j+1}$$

to both sides of the equation. Using Eq. (90) and commutativity of the operators of the form  $\mathcal{D}_a^2 - 1$ , we find

$$\prod_{j=1}^n (\mathcal{D}_{a_j}^2 - 1)^{m_j+1} (\partial_{xx} - \omega)u = \bar{\alpha}\partial_x \prod_{j=1}^n (\mathcal{D}_{a_j}^2 - 1)^{m_j+1} \mathcal{A}u \quad (91)$$

$$= \bar{\alpha}\partial_x \sum_{i=1}^n c_i \left[ \prod_{j=1, j \neq i}^n (\mathcal{D}_{a_j}^2 - 1)^{m_j+1} \mathcal{L}_{m_i}^{a_i} u \right]. \quad (92)$$

This is an ordinary differential equation of degree  $2 + 2 \sum_i (m_i + 1)$ , which a solution  $u$  of the integrodifferential eigenvalue equation has to satisfy. Importantly, not every solution of this ODE also solves the original eigenvalue equation: by taking the derivatives we lose information. The ODE has to be complemented by a set of conditions, as well as the original boundary condition, to fix the solution and also  $\omega$ .

## 6. A few examples

- For the exponential kernel we use in the main text,  $g(x) = g_0^1(x) = e^{-x}$ , we have

$$\mathcal{L}_0^1 = -2\partial_x.$$

Note that  $\mathcal{D}_1$  is just  $\partial_x$ . The ODE is

$$(\partial_{xx} - 1)(\partial_{xx} - \omega)u = -2\bar{\alpha}\partial_{xx}u, \quad (93)$$

or equivalently

$$\partial_x^4 u + (2\bar{\alpha} - 1 - \omega)\partial_x^2 u + \omega u = 0. \quad (94)$$

- For a kernel that is given by a single function  $g(x) = g_m^1(x) = x^m e^{-x}$ , the ODE is

$$(\partial_{xx} - 1)^{m+1} (\partial_{xx} - \omega)u = \bar{\alpha}\partial_x \mathcal{L}_m^1 u \quad (95)$$

with  $\mathcal{L}_m^1$  as in Eq. (87).

- For a kernel that is a combination of two exponentials, for example

$$c_1 g_0^{a_1}(x) + c_2 g_0^{a_2}(x) = c_1 a_1 e^{-a_1 x} + c_2 a_2 e^{-a_2 x},$$

the ODE is

$$(a_1^{-2}\partial_{xx} - 1)(a_2^{-2}\partial_{xx} - 1)(\partial_{xx} - \omega)u = \bar{\alpha}\partial_x (c_1(\mathcal{D}_{a_2}^2 - 1)\mathcal{L}_0^{a_1} + c_2(\mathcal{D}_{a_1}^2 - 1)\mathcal{L}_0^{a_2})u \quad (96)$$

$$= -2\bar{\alpha}(c_1 a_1^{-1}(a_2^{-2}\partial_{xx} - 1)\partial_{xx} + c_2 a_2^{-1}(a_1^{-2}\partial_{xx} - 1)\partial_{xx})u \quad (97)$$

$$= -2\bar{\alpha} \left( \left[ \frac{c_1}{a_1 a_2^2} + \frac{c_2}{a_2 a_1^2} \right] \partial_x^4 - \left[ \frac{c_1}{a_1} + \frac{c_2}{a_2} \right] \partial_{xx} \right) u \quad (98)$$

Multiplying both sides with  $a_1^2 a_2^2$  gives

$$(\partial_{xx} - a_1^2)(\partial_{xx} - a_2^2)(\partial_{xx} - \omega)u = -2\bar{\alpha} ((c_1 a_1 + c_2 a_2)\partial_x^4 - (c_1 a_1 a_2^2 + c_2 a_2 a_1^2)\partial_{xx})u. \quad (99)$$

This result could be particularly useful, since varying the four parameters  $a_1, a_2, c_1, c_2$  produces a range of interaction kernels, possibly with attractive and repulsive parts on different length scales.

## V. SOLUTION FOR THE EIGENVALUES AND EIGENFUNCTIONS WHEN $m = 0$

We now use the ODE formulation of the eigenvalue problem to obtain an algebraic set of equations that determines  $\omega$ . The strategy is to solve the ODE explicitly, and plug the solutions into the original integrodifferential eigenvalue equation as well as the boundary conditions. We only do this for the simplest case of the single exponential. The integral eigenvalue equation is

$$\partial_{xx}u - \bar{\alpha}\partial_x\mathcal{A}_0u = \omega u, \text{ with } (\partial_x - \bar{\alpha}\mathcal{A}_0)u(x) = 0 \quad \text{at } x = 0, x = \ell$$

and the ODE is

$$\partial_x^4 u + (2\bar{\alpha} - \omega - 1)\partial_x^2 u + \omega u = 0. \quad (100)$$

The characteristic equation corresponding to Eq. (100) is the quartic

$$z^4 + (2\bar{\alpha} - 1 - \omega)z^2 + \omega = 0. \quad (101)$$

This is a biquadratic equation, whose solutions  $z$  are given by

$$z = \pm\sqrt{w_1} \quad z = \pm\sqrt{w_2},$$

with  $w_{1,2}$  the two solutions of the quadratic

$$w^2 + (2\bar{\alpha} - 1 - \omega)w + \omega = 0.$$

The solutions depend on  $\bar{\alpha}$  and  $\omega$ , and can be positive, negative, or complex. Depending on this, the real solutions of the ODE are expressed in terms of exponentials and/or sines and cosines.

In the generic case (i.e. for all except isolated values of  $\bar{\alpha}$  and  $\omega$ ), there are two distinct roots  $w_1$  and  $w_2$  of this equation, and four distinct roots  $z_1, z_2, z_3, z_4$  of the quartic. Moreover we can assume  $z_1 = -z_3$  and  $z_2 = -z_4$ .

The general solution of the ODE is

$$u(x) = \sum_i A_i e^{z_i x}.$$

From the parity argument, we know that we only need to consider odd and even solutions of this equation. We can thus restrict the solutions of interest to those expressed as

$$u(x) = A_1(e^{z_1 \hat{x}} + (-1)^n e^{-z_1 \hat{x}}) + A_2(e^{z_2 \hat{x}} + (-1)^n e^{-z_2 \hat{x}}) \quad (102)$$

$$= A_1 f_1^n(x) + A_2 f_2^n(x), \quad (103)$$

where we have defined

$$f_i^n = e^{z_i \hat{x}} + (-1)^n e^{-z_i \hat{x}}.$$

We use the variable  $\hat{x} = x - \ell/2$  which will be easier in the following. At this point,  $A_1$  and  $A_2$  can be complex numbers, and the  $z_i$  too. Eq. (103) contains both the odd ( $n$  odd) and even ( $n$  even) solutions.

Next we require that such a solution satisfies the original integro-differential eigenvalue problem, as well as the boundary conditions. We first calculate  $\mathcal{A}_0(e^{z\hat{x}})$  for general  $z$ :

$$\mathcal{A}_0(e^{z(x-\ell/2)}) = \frac{1}{1-z^2} \left( 2ze^{z\hat{x}} + (1-z)e^{-\frac{\ell z}{2}-x} - (1+z)e^{\frac{\ell z}{2}+x-\ell} \right).$$

From this, we find immediately (by putting  $z \mapsto -z$  and adding/subtracting)

$$\mathcal{A}_0(e^{z\hat{x}} + (-1)^n e^{-z\hat{x}}) = \frac{2z}{1-z^2} (e^{z\hat{x}} - (-1)^n e^{-z\hat{x}}) + h^{n+1}(x)\zeta(z) \quad (104)$$

in which we have defined

$$h^n(x) = e^{x-\ell} + (-1)^n e^{-x} \quad (105)$$

$$\zeta(z) = \frac{e^{\frac{\ell z}{2}}}{z-1} - (-1)^n \frac{e^{-\frac{\ell z}{2}}}{z+1} \quad (106)$$

Note that  $h^n(x)$  has the parity of  $n$  and moreover  $\partial_x h^n(x) = h^{n+1}(x)$ . We also see that  $\partial_x f_i^n = z_i f_i^{n+1}$ , which entails

$$(\partial_x - \bar{\alpha}\mathcal{A}_0)f_i^n = z_i f_i^{n+1} - \bar{\alpha} \left( \frac{2z_i}{1 - z_i^2} f_i^{n+1} + h^{n+1}(x)\zeta(z_i) \right) = \left( z_i - \frac{2\bar{\alpha}z_i}{1 - z_i^2} \right) f_i^{n+1} - \bar{\alpha} h^{n+1}(x)\zeta(z_i) \quad (107)$$

We can simplify the term in brackets, starting from the quartic equation that the  $z_i$  satisfy. We have

$$z^4 + (2\bar{\alpha} - 1 - \omega)z^2 + \omega = z^2(z^2 + 2\bar{\alpha} - 1) + \omega(1 - z^2),$$

such that the quartic equation  $z^4 + (2\bar{\alpha} - 1 - \omega)z^2 + \omega = 0$  implies that

$$\frac{1 - z^2 - 2\bar{\alpha}}{1 - z^2} = \frac{\omega}{z^2},$$

which in turn gives

$$z_i - \bar{\alpha} \frac{2z_i}{1 - z_i^2} = \frac{z_i(1 - z_i^2 - 2\bar{\alpha})}{1 - z_i^2} = \frac{\omega}{z_i}.$$

This piece of algebra thus yields, from Eq. (107),

$$(\partial_x - \bar{\alpha}\mathcal{A}_0)f_i^n = \frac{\omega}{z_i} f_i^{n+1} - \bar{\alpha}\zeta(z_i)h^{n+1}(x). \quad (108)$$

Taking one more  $x$ -derivative (recall  $\partial_x f_i^n = z_i f_i^{n+1}$ , and notice  $f_i^{n+2} = f_i^n$ ) gives

$$(\partial_{xx} - \bar{\alpha}\partial_x\mathcal{A}_0)f_i^n = \omega f_i^n - \bar{\alpha}h^n(x)\zeta(z_i), \quad (109)$$

Or equivalently

$$(\partial_{xx} - \bar{\alpha}\partial_x\mathcal{A}_0 - \omega)f_i^n = -\bar{\alpha}h^n(x)\zeta(z_i) \quad (110)$$

Next, we require that  $A_1 f_1^n + A_2 f_2^n$  is an eigenfunction, i.e.

$$(\partial_{xx} - \bar{\alpha}\partial_x\mathcal{A}_0 - \omega)(A_1 f_1^n + A_2 f_2^n) = 0.$$

Combining the last two equations yields the condition

$$-\bar{\alpha}h^n(x)(A_1\zeta(z_1) + A_2\zeta(z_2)) = 0 \quad (111)$$

or just

$$A_1\zeta(z_1) + A_2\zeta(z_2) = 0. \quad (112)$$

This gives us a relation between  $A_1$  and  $A_2$ .

Next we impose the boundary condition at  $x = 0$ , which will finally constrain the  $z$  and thus the  $\omega$ . Recall that because of the parity, the condition at  $x = 0$  implies the one at  $x = \ell$ . The boundary condition on an eigenfunction  $u$  is

$$(\partial_x - \bar{\alpha}\mathcal{A}_0)u = 0 \quad \text{at } x = 0.$$

From Eq. (108), we have

$$(\partial_x - \bar{\alpha}\mathcal{A}_0)f_i^n = \frac{\omega}{z_i} f_i^{n+1} - \bar{\alpha}\zeta(z_i)h^{n+1}(x) \quad (113)$$

For a general eigenfunction, we thus find

$$(\partial_x - \bar{\alpha}\mathcal{A}_0)(A_1 f_1^n + A_2 f_2^n) = A_1 \left( \frac{\omega}{z_1} f_1^{n+1} - \bar{\alpha}\zeta(z_1)h^{n+1}(x) \right) + A_2 \left( \frac{\omega}{z_2} f_2^{n+1} - \bar{\alpha}\zeta(z_2)h^{n+1}(x) \right) \quad (114)$$

$$= \omega \left( A_1 \frac{f_1^{n+1}}{z_1} + A_2 \frac{f_2^{n+1}}{z_2} \right) - \bar{\alpha}(A_1\zeta(z_1) + A_2\zeta(z_2))h^{n+1}(x) \quad (115)$$

$$= \omega \left( A_1 \frac{f_1^{n+1}}{z_1} + A_2 \frac{f_2^{n+1}}{z_2} \right), \quad (116)$$



where the last part drops out because of the condition Eq. (112) derived above. The boundary condition requires this expression to be equal to zero when evaluated at  $x = 0$ :

$$\omega \left( A_1 \frac{f_1^{n+1}(0)}{z_1} + A_2 \frac{f_2^{n+1}(0)}{z_2} \right) = 0 \quad (117)$$

Now  $f_i^{n+1}(0) = e^{-\frac{z_i \ell}{2}} - (-1)^n e^{\frac{z_i \ell}{2}}$ . Let us define, again for convenience,

$$\gamma(z) = \frac{e^{-\frac{z \ell}{2}} - (-1)^n e^{\frac{z \ell}{2}}}{z}. \quad (118)$$

With these definitions, the boundary condition Eq. (117) can be written as (if  $\omega \neq 0$ )

$$A_1 \gamma(z_1) + A_2 \gamma(z_2) = 0. \quad (119)$$

Eq. (112) and Eq. (119) together constitute a system of two linear equations for  $A_1$  and  $A_2$ , which can be written in matrix form as

$$\begin{pmatrix} \zeta(z_1) & \zeta(z_2) \\ \gamma(z_1) & \gamma(z_2) \end{pmatrix} \begin{pmatrix} A_1 \\ A_2 \end{pmatrix} = \begin{pmatrix} 0 \\ 0 \end{pmatrix} \quad (120)$$

In order for a non-zero eigenfunction  $u$  to exist, the determinant of this matrix has to be zero, which will be the equation fixing  $\omega$ . Finally, we have the following set of equations:

$$\begin{aligned} z_1^4 + (2\bar{\alpha} - 1 - \omega)z_1^2 + \omega &= 0 \\ z_2^4 + (2\bar{\alpha} - 1 - \omega)z_2^2 + \omega &= 0 \\ \zeta(z_1)\gamma(z_2) - \zeta(z_2)\gamma(z_1) &= 0. \end{aligned} \quad (121)$$

It is important to take  $z_1$  and  $z_2$  that correspond to the two *different* roots  $w$  of the quadratic equation. We can also write the equations in terms of the  $w_i$ :

$$\begin{aligned} w_1^2 + (2\bar{\alpha} - 1 - \omega)w_1 + \omega &= 0 \\ w_2^2 + (2\bar{\alpha} - 1 - \omega)w_2 + \omega &= 0 \\ \zeta(\sqrt{w_1})\gamma(\sqrt{w_2}) - \zeta(\sqrt{w_2})\gamma(\sqrt{w_1}) &= 0. \end{aligned} \quad (122)$$

After fixing either  $\ell$ , this is a set of four equations for the variables  $z_1, z_2, \bar{\alpha}$  and  $\omega$ , which defines curves in the  $(\bar{\alpha}, \omega)$ -plane, shown in Fig. ???. For any solution, one can construct the eigenfunction by explicitly solving for  $A_1, A_2$  and normalizing such that the eigenfunction is real.

#### A. Determining parameter values for which $\omega = 0$

To determine an analytical expression that defines the instability curves in Fig. 2 in the main text, we impose  $\omega = 0$  and extract conditions on  $L$  and  $\bar{\alpha}$ .

If  $\omega = 0$ , the fourth order ODE is

$$\partial_x^4 u + (2\bar{\alpha} - 1)\partial_x^2 u = 0 \quad (123)$$

which integrated twice becomes

$$\partial_{xx} u + (2\bar{\alpha} - 1)u = ax + b \quad (124)$$

The general solution of this equation is

$$u(x) = a'x + b' + Ae^{zx} + Be^{-zx} \quad (125)$$

for constants  $a', b', A, B$  and where  $z$  satisfies  $z^2 = 1 - 2\bar{\alpha}$ . The even solutions are of the form

$$u(x) = A + B(e^{z\hat{x}} + e^{-z\hat{x}}) \quad (126)$$

and odd solutions are of the form

$$A\hat{x} + B(e^{z\hat{x}} - e^{-z\hat{x}}), \quad (127)$$

with  $\hat{x} = x - \ell/2$  as before. Now we impose that these solutions satisfy the integro-differential eigenvalue equation as well as the boundary conditions. First, we calculate

$$\mathcal{A}_0(1) = -(e^{x-\ell} - e^{-x}) = -h^1(x) \quad (128)$$

$$\mathcal{A}_0(\hat{x}) = 2 - \frac{\ell+2}{2}(e^{x-\ell} + e^{-x}) = 2 - \frac{\ell+2}{2}h^2(x). \quad (129)$$

Denoting  $f^n(x) = e^{z\hat{x}} + (-1)^n e^{-z\hat{x}}$ , we have for the even solutions (using Eq. (108) with  $\omega = 0$ )

$$\begin{aligned} (\partial_x - \bar{\alpha}\mathcal{A}_0)(A + Bf^0) &= -\bar{\alpha}A\mathcal{A}_0(1) + B(-\bar{\alpha}\zeta(z)h^1(x)) \\ &= A\bar{\alpha}h^1(x) - B\bar{\alpha}\zeta(z)h^1(x). \end{aligned}$$

and thus

$$(\partial_{xx} - \bar{\alpha}\partial_x\mathcal{A}_0)(A + Bf^0) = \bar{\alpha}h^0(x)(A - B\zeta(z)).$$

The eigenvalue equation (and immediately the boundary condition) are satisfied for

$$A = B\zeta(z).$$

Generically this gives a set of eigenfunctions of  $\omega = 0$  that are due to the mass-conservation of the system, givne by

$$u(x) = \zeta(z) + e^{z\hat{x}} + e^{-z\hat{x}}, \quad z^2 = 1 - 2\bar{\alpha}$$

Importantly, there are other solutions that exist only for specific parameter values: namely those for which  $A = 0$  above. A nonzero solution then requires that

$$\zeta(z) = 0$$

Now for the odd solutions of the form  $A\hat{x} + Bf^1(x)$ . We have

$$(\partial_x - \bar{\alpha}\mathcal{A}_0)(A\hat{x} + Bf^1) = A\left(1 - \bar{\alpha}(2 - \frac{\ell+2}{2}h^2(x))\right) + B(-\bar{\alpha}\zeta(z)h^2(x)), \quad (130)$$

one more  $x$ -derivative then gives

$$(\partial_{xx} - \bar{\alpha}\partial_x\mathcal{A}_0)(A\hat{x} + Bf^1) = A\alpha\frac{\ell+2}{2}h^1(x) - B\bar{\alpha}\zeta(z)h^1(x). \quad (131)$$

The latter expression needs to be equal to zero, imposing

$$A\frac{\ell+2}{2} = B\zeta(z)$$

In this case the boundary condition yields

$$A\left(1 - \bar{\alpha}(2 - \frac{\ell+2}{2}h^2(0))\right) + B(-\bar{\alpha}\zeta(z)h^2(0)) = 0,$$

or

$$A(1 - 2\bar{\alpha}) + \left(A\frac{\ell+2}{2} + \zeta(z)B\right)h^2(0) = 0,$$

which entails  $A(1 - 2\bar{\alpha}) = 0$ . Generically we thus have  $A = 0$ , and for a nonzero eigenmode the condition above then means that  $\zeta(z) = 0$ . The other possibility here is that  $1 - 2\bar{\alpha} = 0$ . However, in this case, the original ODE would be  $u'''' = 0$ . Solutions of this equation are no solutions of the original integrodifferential equation and boundary conditions.

Thus, the condition that determines the parameters  $\bar{\alpha}$  and  $\ell$  for which  $\omega = 0$  is an eigenvalue is

$$\zeta(\sqrt{1 - 2\bar{\alpha}}) = 0 \quad (132)$$

where the square root could be real or imaginary.

### 1. Analysis of $\zeta(z) = 0$

The instability lines are obtained by solving  $z^2 = 1 - 2\bar{\alpha}$  and  $\zeta(z) = 0$  together. We can rewrite  $\zeta(z) = 0$  as

$$(-1)^n e^{\ell z} = \frac{z-1}{z+1}. \quad (133)$$

By examining the graphs of the left-hand side and right-hand side, we see that the only possible real solution is  $z = 0$  for  $n$  odd. But  $z = 0$  would imply  $\bar{\alpha} = 1/2$ , which is impossible as we've seen before. Thus, only imaginary solutions are possible, corresponding to  $\bar{\alpha} > 1/2$ .

### 2. Plotting the curves in the $\ell, \bar{\alpha}$ plane.

The equation  $\zeta(\sqrt{1-2\bar{\alpha}})$  defines a collection of curves in the  $\ell, \bar{\alpha}$  plane. We can plot them either as the zero-contours of  $\zeta$ , or we can use a parametrization of the curves as follows.

The condition on  $z$  can be rewritten as

$$e^{i(n\pi+\ell x)} = (-1)^n e^{\ell i x} = \frac{i x - 1}{i x + 1} \quad (134)$$

for real  $x$  (because we need  $z$  to be imaginary). Note that both sides map  $x$  to a point on the unit circle in the complex plane. To draw curves in the  $(\ell, \bar{\alpha})$  plane we use a parametrization  $\ell(\theta), \bar{\alpha}(\theta)$  where  $\theta$  determines a point on the unit circle  $e^{i\theta}$ . Fix  $\theta$ , then compute

$$x = -i \frac{1 + e^{i\theta}}{1 - e^{i\theta}}. \quad (135)$$

From  $z$  we know the value of  $\bar{\alpha}$  as  $\frac{1}{2}(1 - z^2)$ . To compute  $\ell$ , we use

$$e^{i(n\pi+\ell x)} = e^{i\theta}$$

such that  $\ell = (\theta - n\pi)/x$ .

## VI. DETAILS ON THE PERTURBATION METHOD

This method is inspired by a technique from quantum mechanics, namely to solve the Schrödinger equation for a potential which is a small perturbation of an “easy” potential. Then, the energy levels (eigenvalues) can be obtained as a power series in a small parameter  $\epsilon$ . We write the eigenvalue equation, and set  $\bar{\alpha} = \epsilon$  which will be the small parameter:

$$(\partial_{xx} - \epsilon \partial_x \mathcal{A})u = \omega u, \quad (\partial_x - \epsilon \mathcal{A})(u)(x) = 0 \text{ at } x = 0, x = \ell$$

Note that the parameter  $\epsilon$  also appears in the boundary condition.

We write the solution of the full problem as a power series in  $\epsilon$ :

$$u(x) = u_0(x) + \epsilon u_1(x) + \epsilon^2 u_2(x) + \dots, \quad \omega = \omega_0 + \epsilon \omega_1 + \epsilon^2 \omega_2 + \dots \quad (136)$$

Substituting this expression into the equation and keeping terms up to order  $\epsilon$  gives

$$\partial_{xx} u_0 + \epsilon (\partial_{xx} u_1 - \partial_x \mathcal{A} u_0) = \omega_0 u_0 + \epsilon (\omega_1 u_0 + \omega_0 u_1) + \mathcal{O}(\epsilon^2) \quad (137)$$

with boundary condition: at  $x = 0$  and  $x = \ell$  we require

$$\partial_x u_0 + \epsilon (\partial_x u_1 - \mathcal{A} u_0) = \mathcal{O}(\epsilon^2). \quad (138)$$

Now, we proceed by comparing the terms multiplying the different powers of  $\epsilon$ . The problem of order  $\epsilon^0$  is

$$\partial_{xx} u_0 = \omega_0 u_0, \quad \partial_x u_0 = 0 \text{ at } x = 0, \ell. \quad (139)$$

The solutions of this equation are well known, we have for the eigenfunctions and eigenvalues

$$u_0(x) = \cos \frac{n\pi}{\ell} x, \quad \omega_0 = -\left(\frac{n\pi}{\ell}\right)^2 \quad \text{for } n = 0, 1, 2, \dots \quad (140)$$

Note that for each  $n$  we have an eigenvalue/eigenfunction pair. In principle the perturbation calculation is to be done separately for each  $n$  but we can do this in one go. The problem of order  $\epsilon$  is

$$\partial_{xx} u_1 - \partial_x \mathcal{A} u_0 = \omega_0 u_1 + \omega_1 u_0, \quad \text{with } \partial_x u_1 - \mathcal{A} u_0 = 0 \text{ at } x = 0, x = \ell. \quad (141)$$

Rewriting the equation gives

$$(\partial_{xx} - \omega_0) u_1 = \omega_1 u_0 + \partial_x \mathcal{A} u_0. \quad (142)$$

We don't need to solve explicitly for  $u_1$  to obtain the expression for  $\omega_1$ : we multiply both sides of Eq. (142) with  $u_0$  and integrate over the interval  $[0, \ell]$  to find

$$\int_0^\ell u_0(x) u_1''(x) dx - \omega_0 \int_0^\ell u_0(x) u_1(x) dx = \omega_1 \int_0^\ell u_0^2(x) dx + \int_0^\ell u_0(x) (\mathcal{A} u_0)'(x) dx. \quad (143)$$

where we use primes instead of  $\partial_x$ . Integration by parts gives

$$\int_0^\ell u_1''(x) u_0(x) dx = u_0 u_1'|_0^\ell - \int_0^\ell u_0'(x) u_1'(x) dx \quad (144)$$

$$= u_0 u_1'|_0^\ell - u_0' u_1|_0^\ell + \int_0^\ell u_0''(x) u_1(x) dx \quad (145)$$

$$= u_0 u_1'|_0^\ell + \omega_0 \int_0^\ell u_0(x) u_1(x) dx. \quad (146)$$

In the last equality we have used the boundary condition on  $u_0$ , as well as  $u_0'' = \omega_0 u_0$ .

We also have

$$\int_0^\ell u_0(x) (\mathcal{A} u_0)'(x) dx = u_0 \mathcal{A} u_0|_0^\ell - \int_0^\ell u_0'(x) \mathcal{A} u_0(x) dx \quad (147)$$

$$= u_0 u_1'|_0^\ell - \int_0^\ell u_0'(x) (\mathcal{A} u_0)(x) dx \quad (148)$$

where in the last equality we used the boundary condition on  $u_1$ .

Substituting Eq. (146) and Eq. (148) into Eq. (143) gives

$$u_0 u_1'|_0^\ell + \omega_0 \int_0^\ell u_0(x) u_1(x) dx - \omega_0 \int_0^\ell u_0(x) u_1(x) dx = \omega_1 \int_0^\ell u_0^2(x) dx + u_0 u_1'|_0^\ell - \int_0^\ell u_0'(x) (\mathcal{A} u_0)(x) dx \quad (149)$$

or, canceling what has to be canceled:

$$0 = \omega_1 \int_0^\ell u_0(x)^2 dx - \int_0^\ell u_0'(x) \mathcal{A} u_0(x) dx. \quad (150)$$

This gives us a solution for the first correction to the eigenvalue:

$$\omega_1 = \frac{\int_0^\ell u_0'(x) (\mathcal{A} u_0)(x) dx}{\int_0^\ell u_0^2(x) dx}. \quad (151)$$

### A. Formula for exponential kernel

For the exponential interaction kernel, we can compute the integrals analytically. We know that  $u_0(x) = \cos(n\pi/\ell x)$ , such that

$$\int_0^\ell u_0^2(x) dx = \int_0^\ell \cos^2\left(\frac{\pi}{\ell} x\right) dx = \begin{cases} \ell/2 & \text{if } n \neq 0 \\ \ell & \text{otherwise} \end{cases} \quad (152)$$

For  $n = 0$ , the eigenvalue is zero always so we continue with  $n \geq 1$ . Using the symbolic algebra package `sympy` for Python, we obtain

$$\begin{aligned} \int_0^\ell u'_0(x)(\mathcal{A}u_0)(x)dx &= \frac{\ell(\pi n)^2}{(\ell^2 + (\pi n)^2)^2} (2\ell e^{-\ell}(-1)^n + \ell^2 - 2\ell + (\pi n)^2) \\ &= \frac{-\omega_0}{(1 - \omega_0)^2} \ell \left( 1 - \omega_0 - \frac{2}{\ell}(1 - (-1)^n e^{-\ell}) \right) \end{aligned} \quad (153)$$

where we used  $\omega_0 = -(n\pi/\ell)^2$ . Finally this gives

$$\omega_1 = \frac{-2\omega_0}{(1 - \omega_0)^2} \left( 1 - \omega_0 - \frac{2}{\ell}(1 - (-1)^n e^{-\ell}) \right) \quad (154)$$

And thus, for the approximation of the eigenvalue  $\omega^n$ :

$$\omega^n = \omega_0^n + \epsilon \omega_1^n + \mathcal{O}(\epsilon^2) = \omega_0 \left( 1 - \frac{2\epsilon}{(1 - \omega_0)^2} \left( 1 - \omega_0 - \frac{2}{\ell}(1 - (-1)^n e^{-\ell}) \right) \right) + \mathcal{O}(\epsilon^2). \quad (155)$$

- 
- [1] Zhao et al., in preparation.
  - [2] Y. Imuta, H. Kiyonari, C. W. Jang, R. R. Behringer, and H. Sasaki, Generation of knock-in mice that express nuclear egfp and tamoxifen-inducible cre recombinase in the notochord from *foxa2* and *t* loci, *Genesis* (New York, N.Y. : 2000) **51**, 210 (2013).
  - [3] T. Abe, H. Kiyonari, G. Shioi, K. I. Inoue, K. Nakao, S. Aizawa, and T. Fujimori, Establishment of conditional reporter mouse lines at *rosa26* locus for live cell imaging, *Genesis* (New York, N.Y. : 2000) **49**, 579 (2011).
  - [4] M. Weigert, U. Schmidt, R. Haase, K. Sugawara, and G. Myers, Star-convex polyhedra for 3d object detection and segmentation in microscopy, 2020 IEEE Winter Conference on Applications of Computer Vision (WACV) , 3655 (2020).
  - [5] S. Berg, D. Kutra, T. Kroeger, C. N. Straehle, B. X. Kausler, C. Haubold, M. Schiegg, J. Ales, T. Beier, M. Rudy, K. Eren, J. I. Cervantes, B. Xu, F. Beuttenmueller, A. Wolny, C. Zhang, U. Koethe, F. A. Hamprecht, and A. Kreshuk, ilastik: interactive machine learning for (bio)image analysis, *Nature Methods* 2019 16:12 **16**, 1226 (2019).
  - [6] A. Gerisch, On the approximation and efficient evaluation of integral terms in PDE models of cell adhesion, *IMA Journal of Numerical Analysis* **30**, 173 (2010).
  - [7] EMBL, J. Pečar, R. Lueck, and M. Wahlers, EMBL Heidelberg HPC Cluster 10.5281/zenodo.12785830 (2020).
  - [8] L. N. Trefethen, *Spectral Methods in MATLAB*, Software, Environments, and Tools (Society for Industrial and Applied Mathematics, 2000).
  - [9] Y. Kuznetsov, *Elements of Applied Bifurcation Theory*, 3rd ed., Applied Mathematical Sciences (Springer-Verlag, New York, 2004).
  - [10] R. Seydel, *Practical Bifurcation and Stability Analysis*, Interdisciplinary Applied Mathematics, Vol. 5 (Springer, New York, NY, 2010).
  - [11] E. F. Keller and L. A. Segel, Initiation of slime mold aggregation viewed as an instability, *Journal of Theoretical Biology* **26**, 399 (1970).
  - [12] K. J. Painter, Mathematical models for chemotaxis and their applications in self-organisation phenomena, *Journal of Theoretical Biology Celebrating the 60th Birthday of Professor Philip Maini*, **481**, 162 (2019).
  - [13] J. S. Bois, F. Jülicher, and S. W. Grill, Pattern Formation in Active Fluids, *Physical Review Letters* **106**, 028103 (2011).
  - [14] K. H. Palmquist, S. F. Tiemann, F. L. Ezzeddine, S. Yang, C. R. Pfeifer, A. Erzberger, A. R. Rodrigues, and A. E. Shyer, Reciprocal cell-ECM dynamics generate supracellular fluidity underlying spontaneous follicle patterning, *Cell* **185**, 1960 (2022).
  - [15] T. J. Jewell, A. L. Krause, P. K. Maini, and E. A. Gaffney, Patterning of nonlocal transport models in biology: The impact of spatial dimension, *Mathematical Biosciences* **366**, 109093 (2023).
